# Supplementary material for: The most variable VVV sources: eruptive protostars, dipping giants in the Nuclear Disc and others
Source: arXiv:2401.14471 ancillary file (2024-01-25)

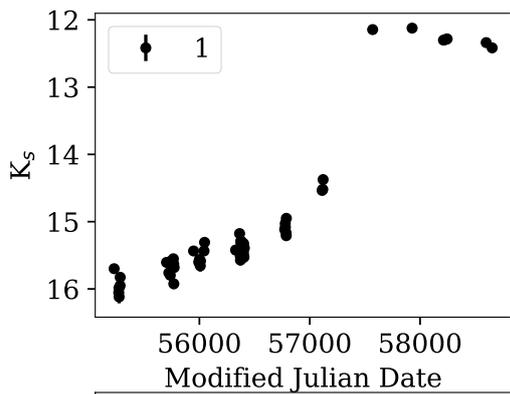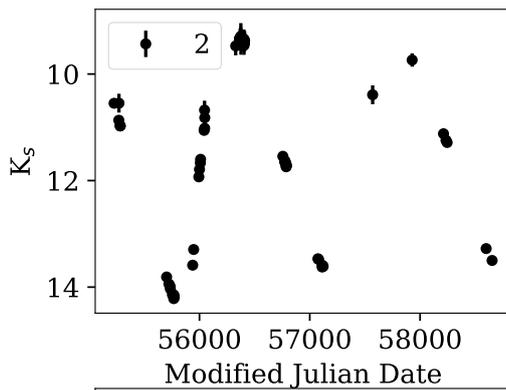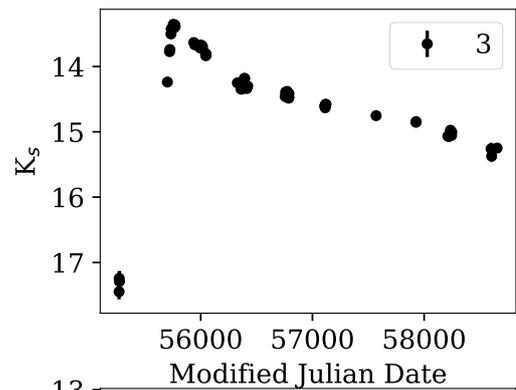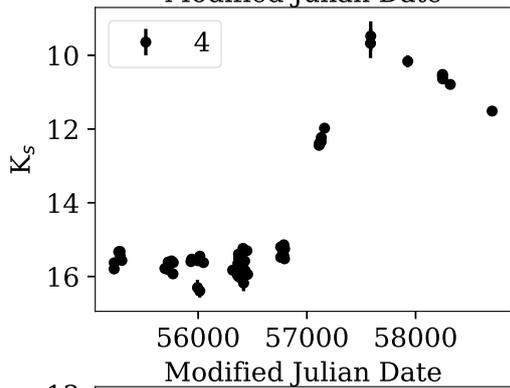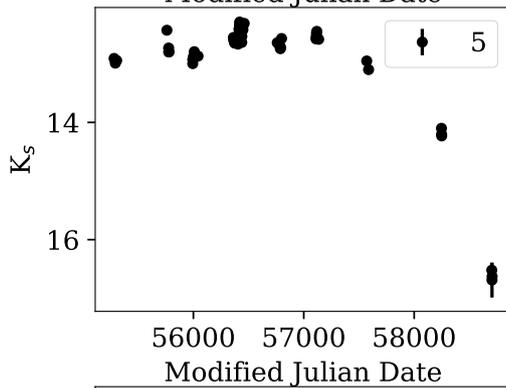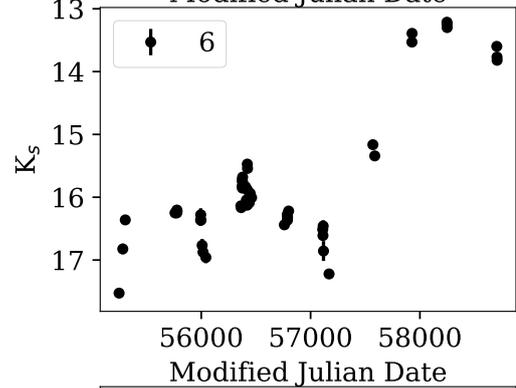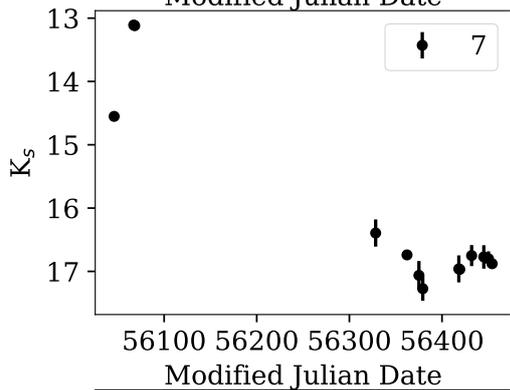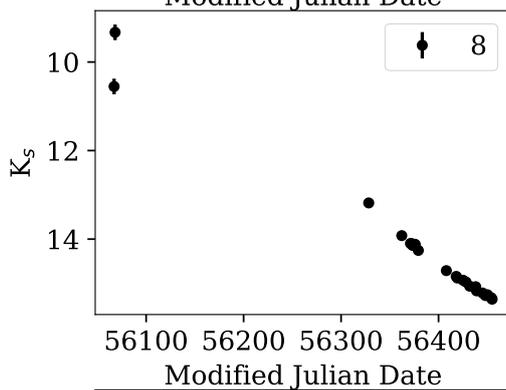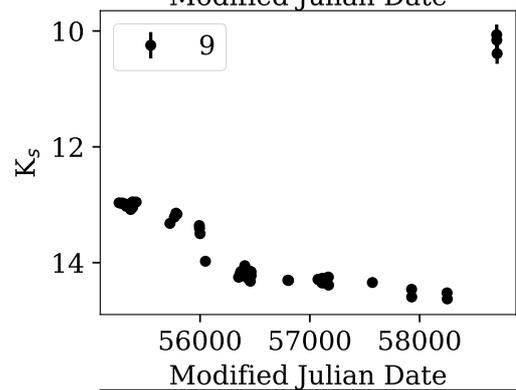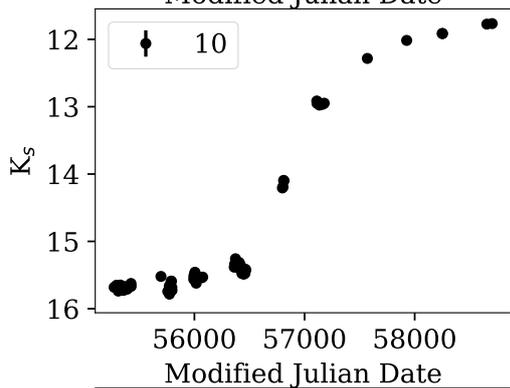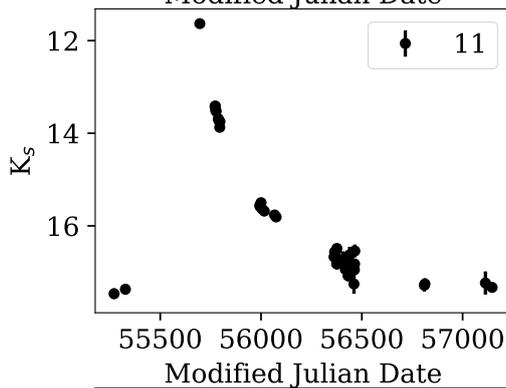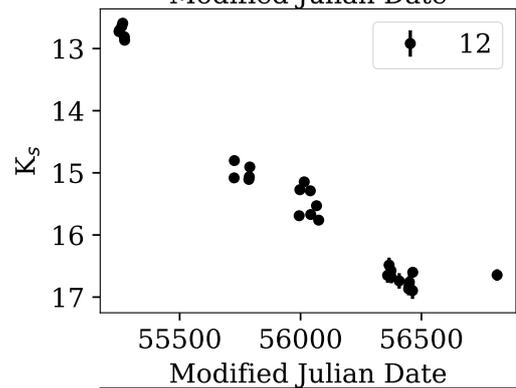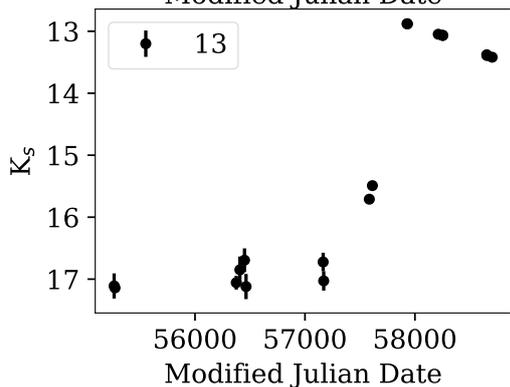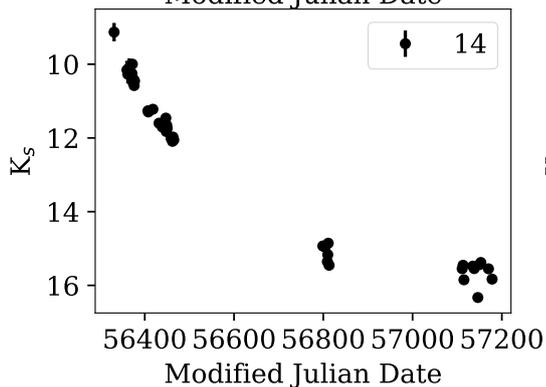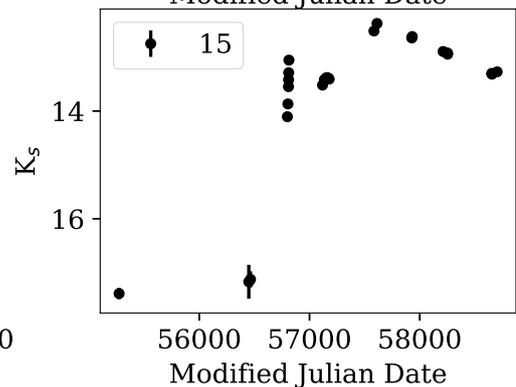

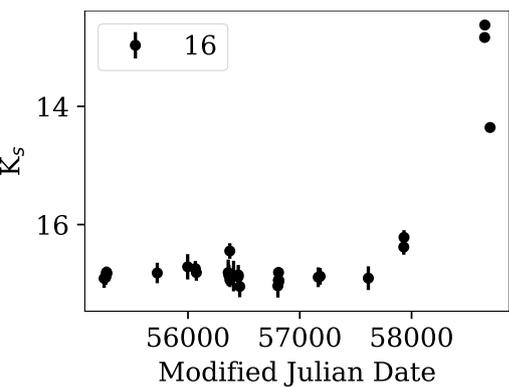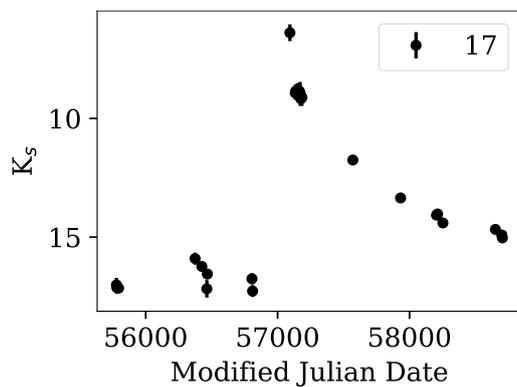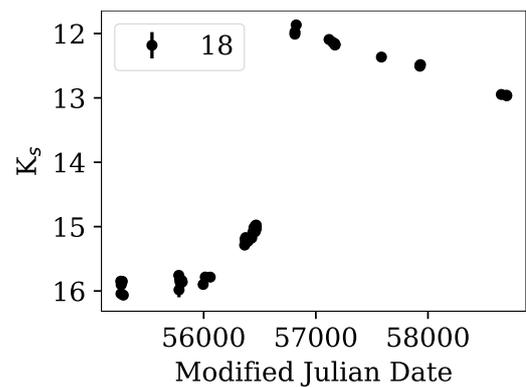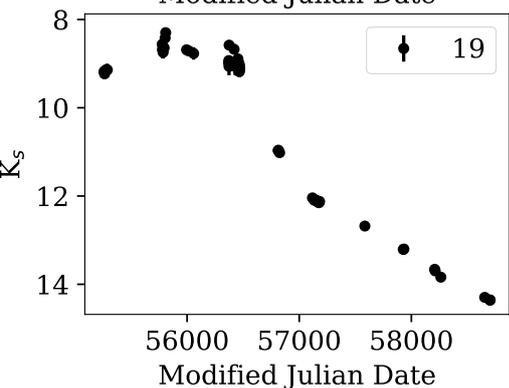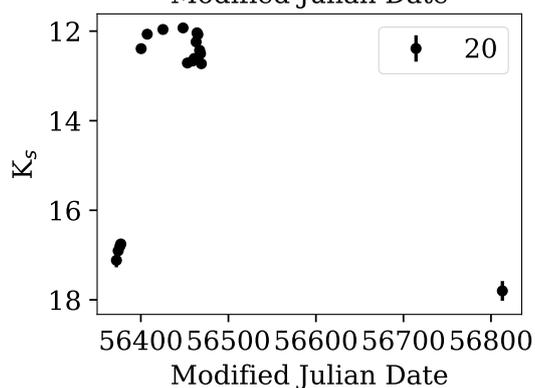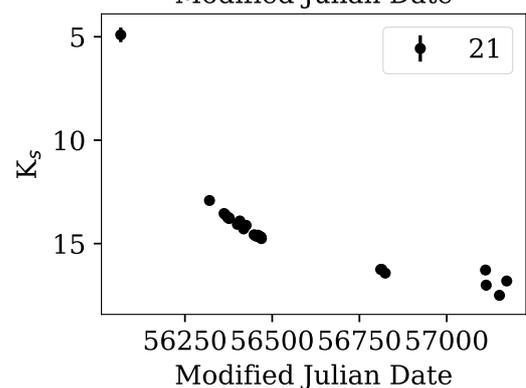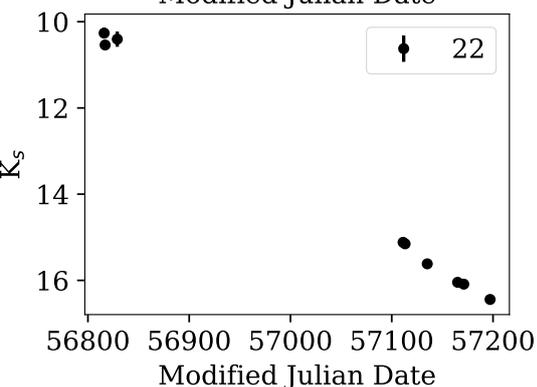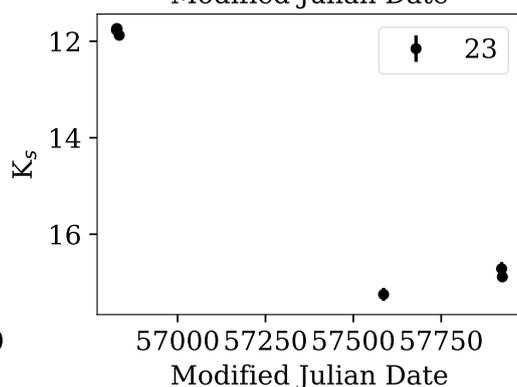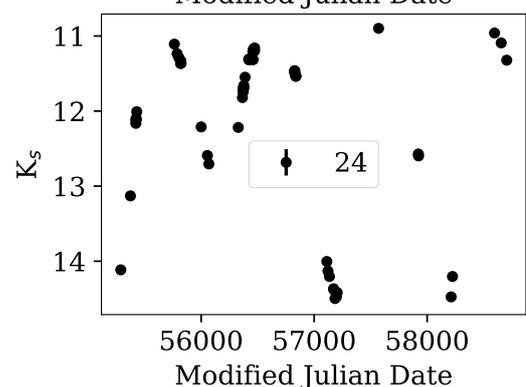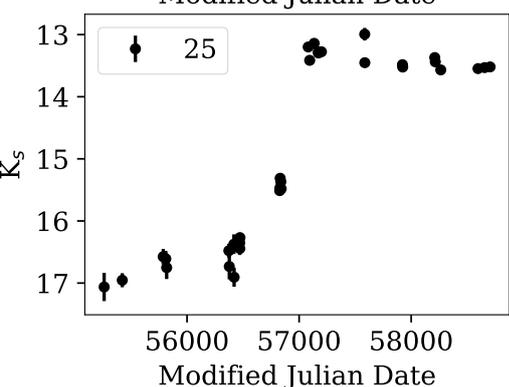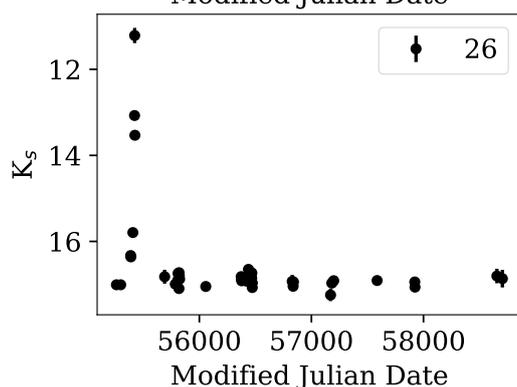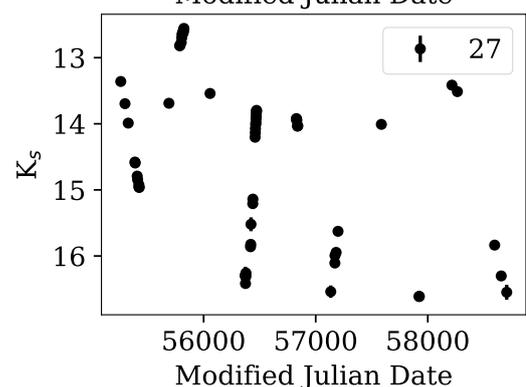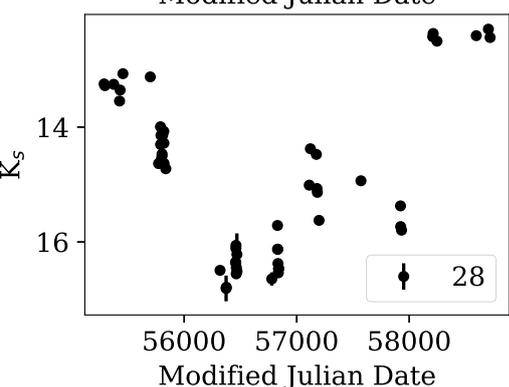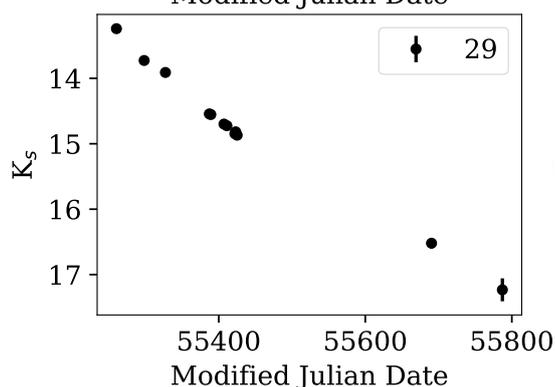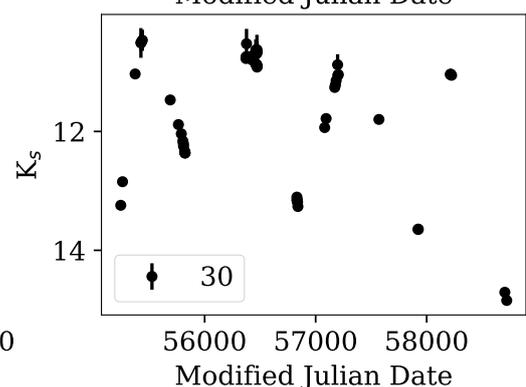

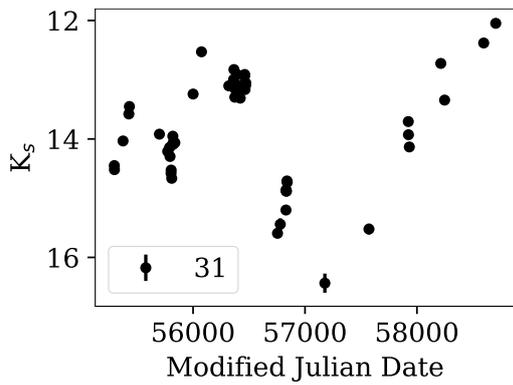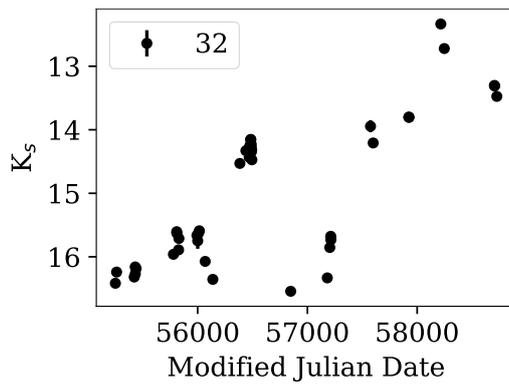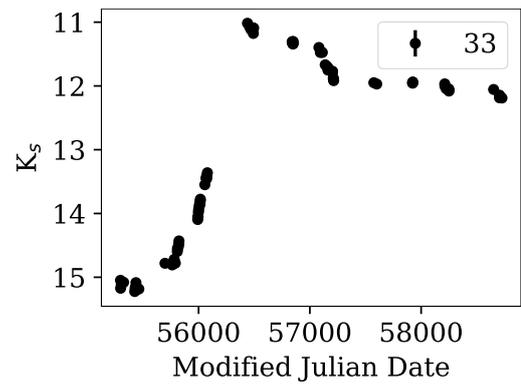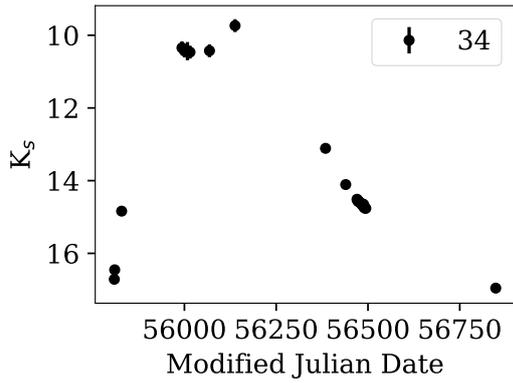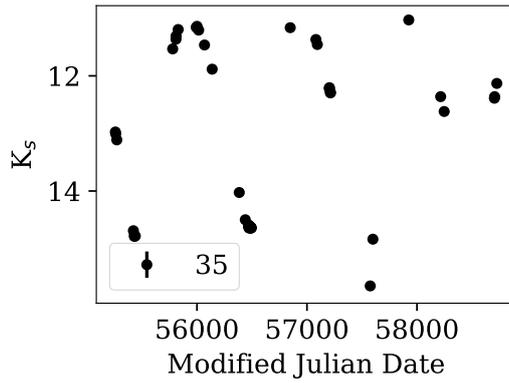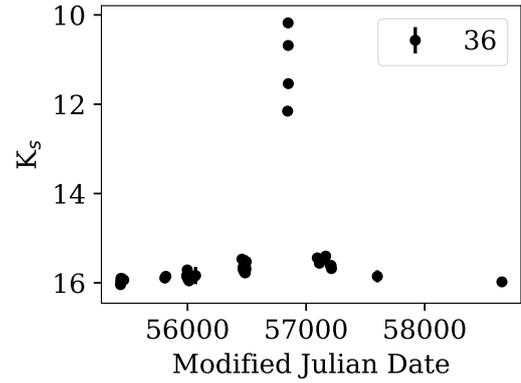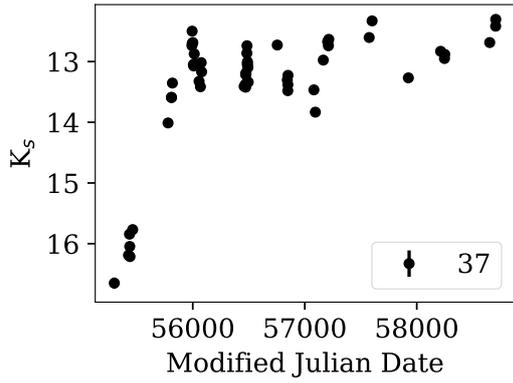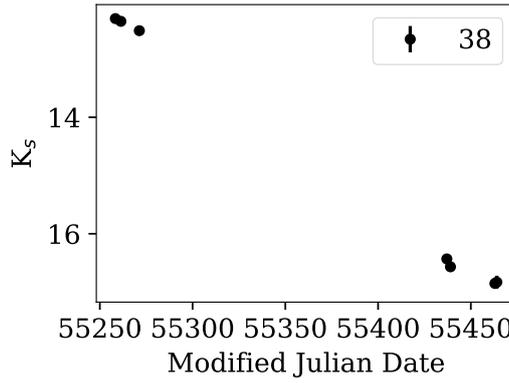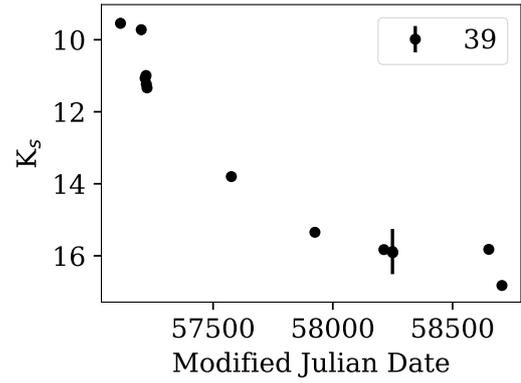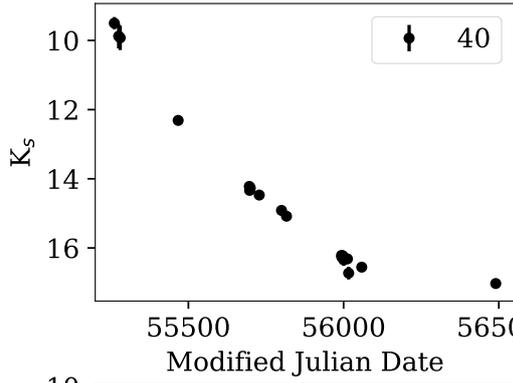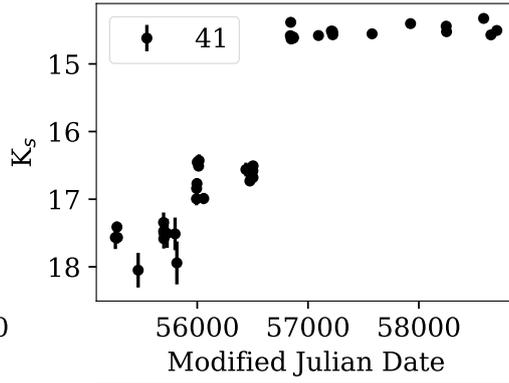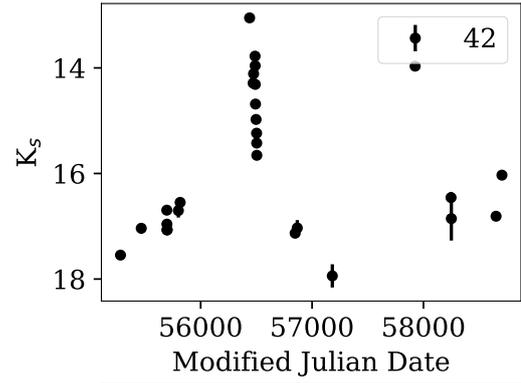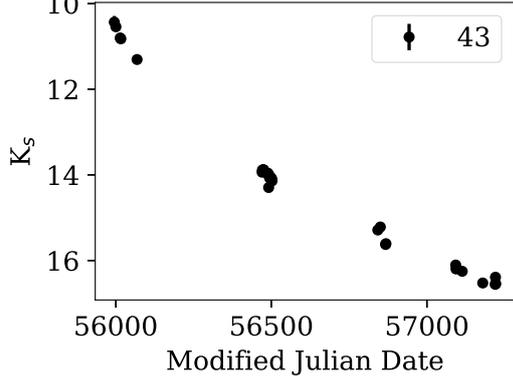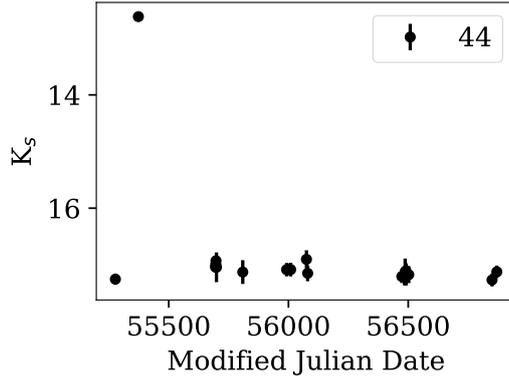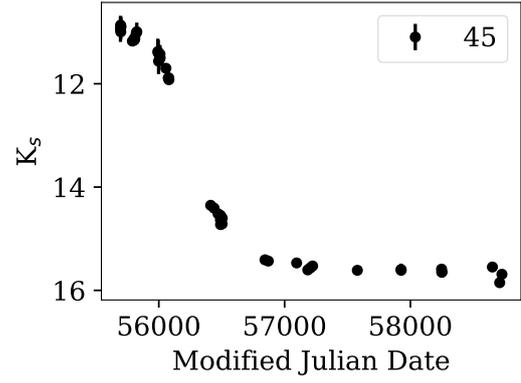

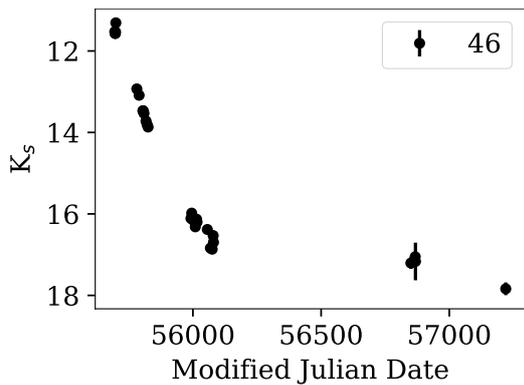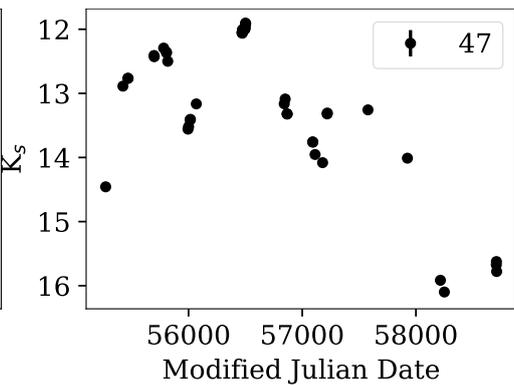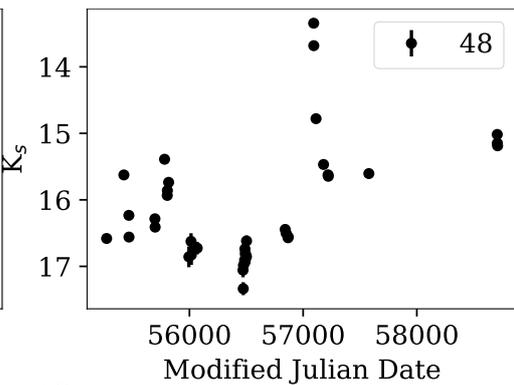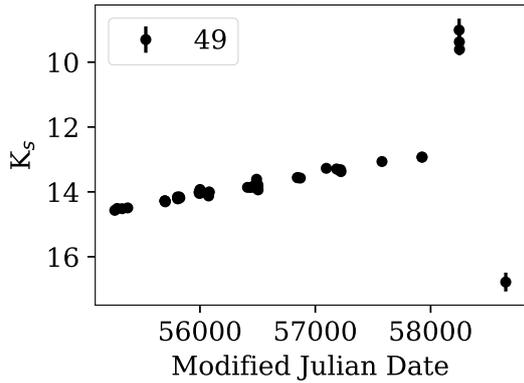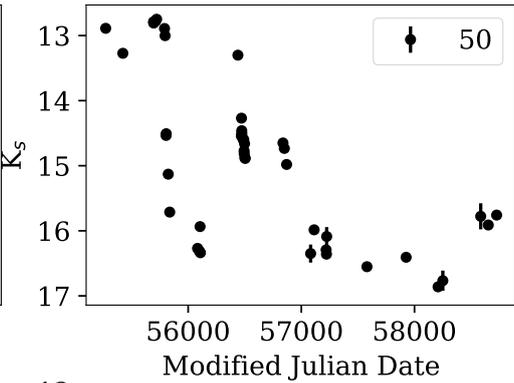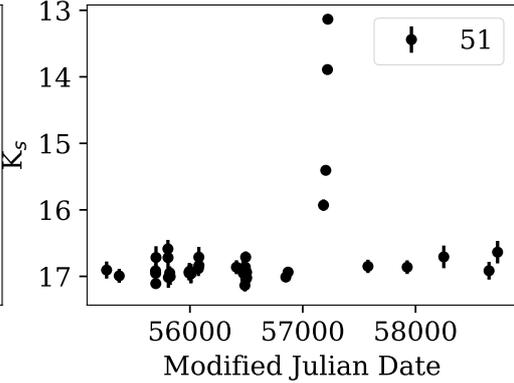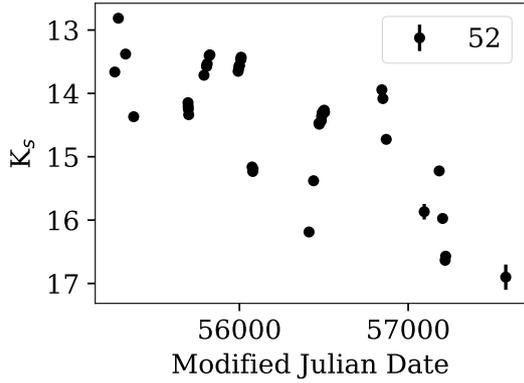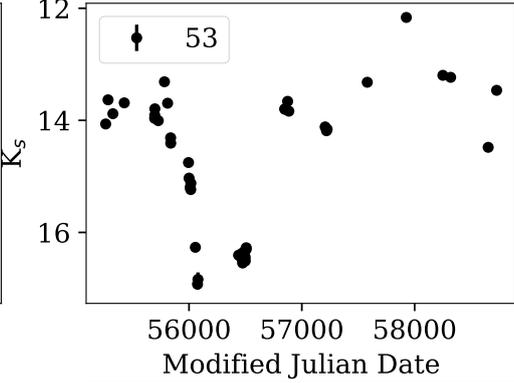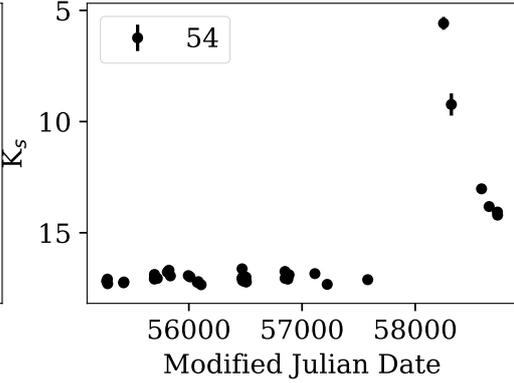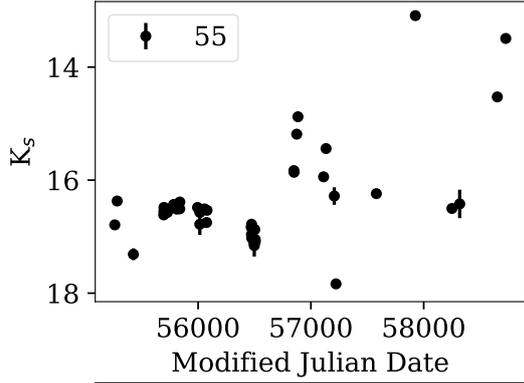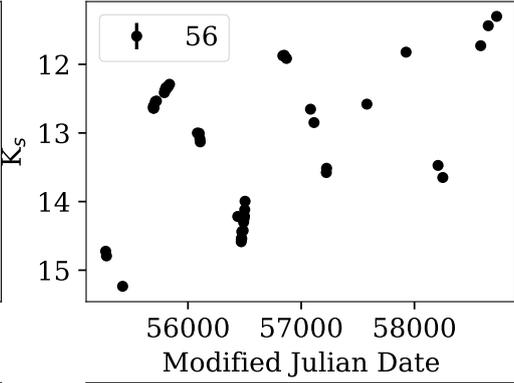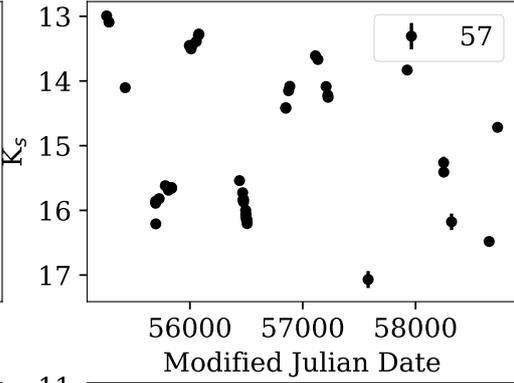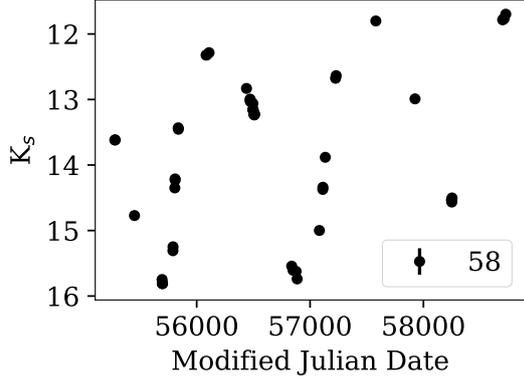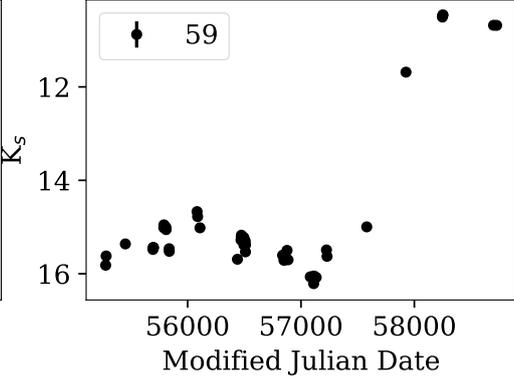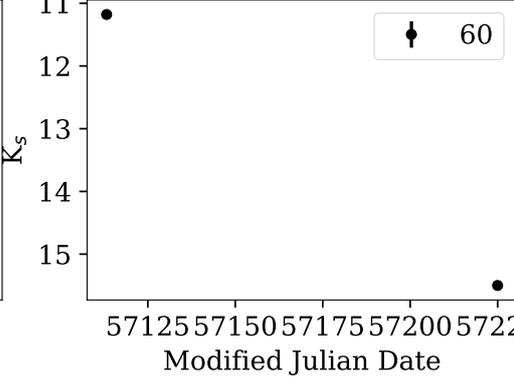

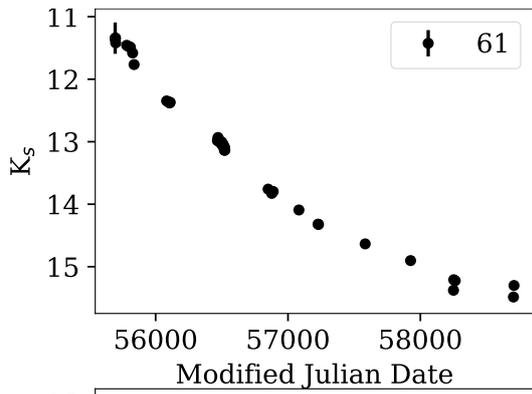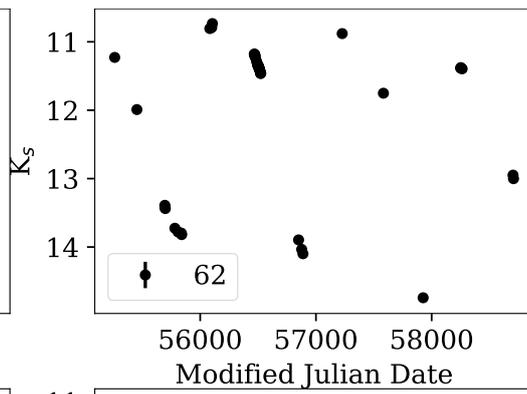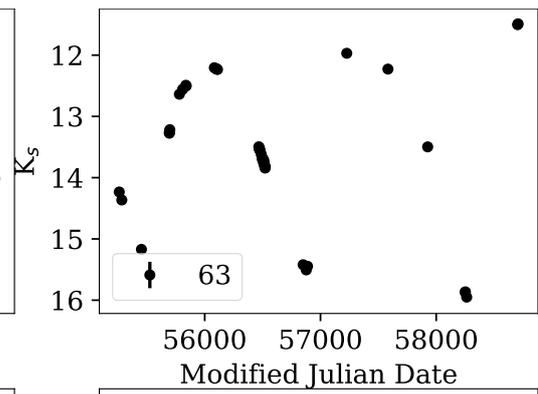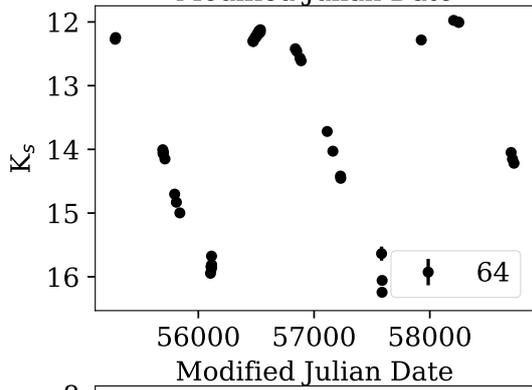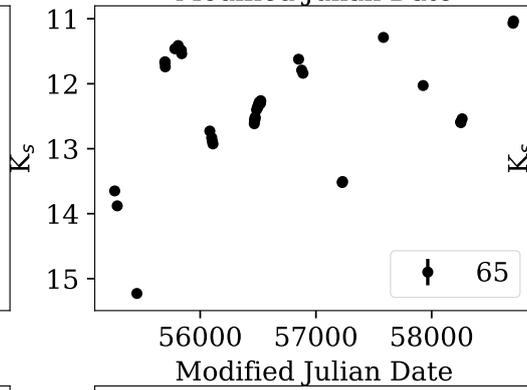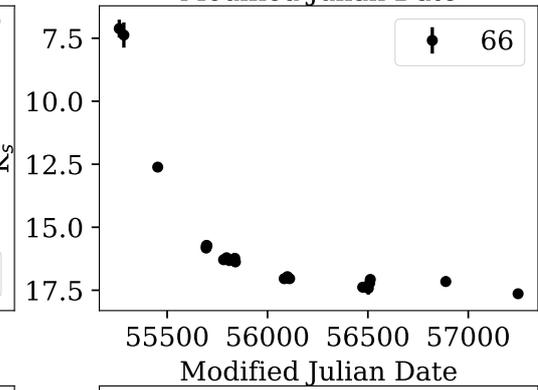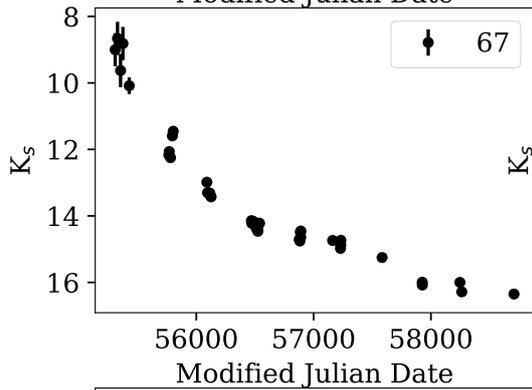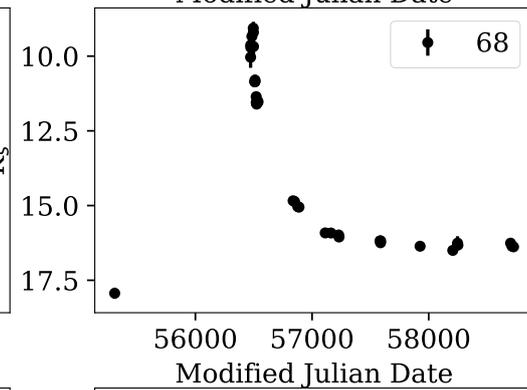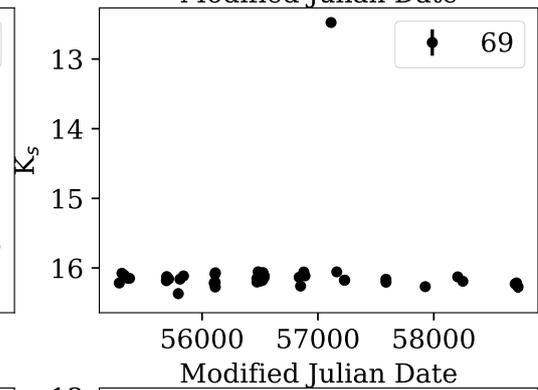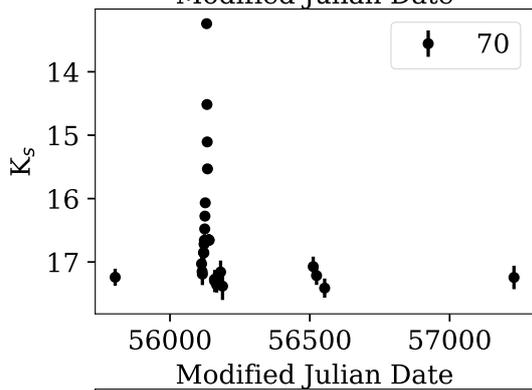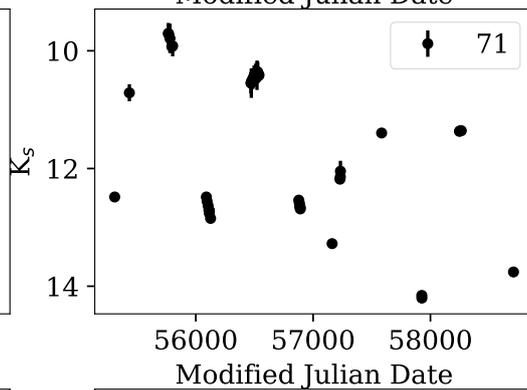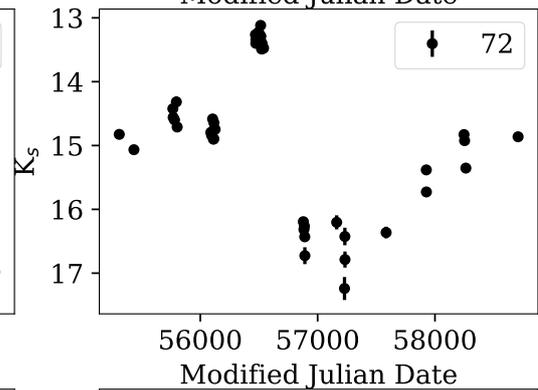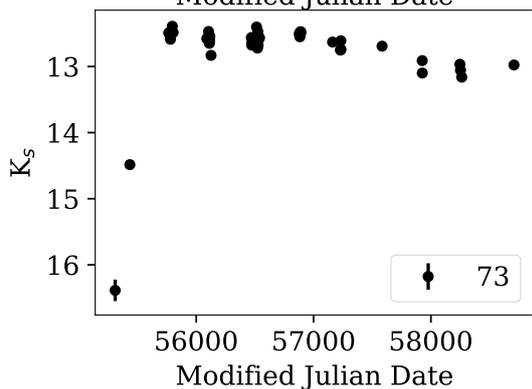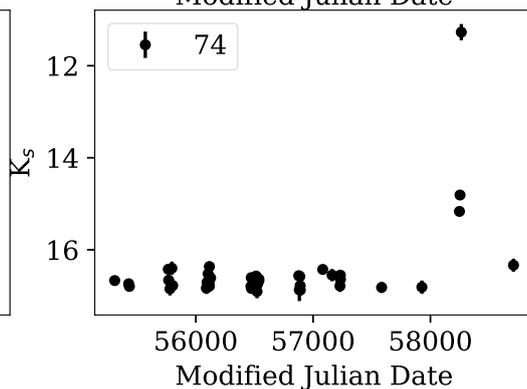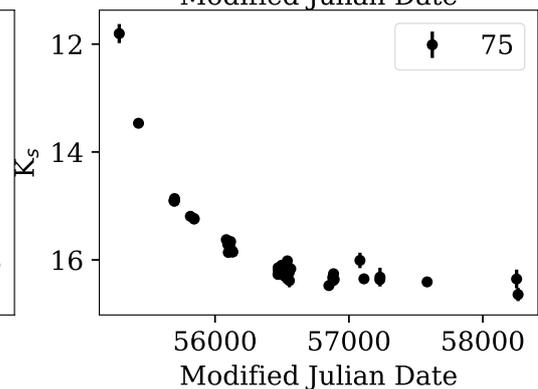

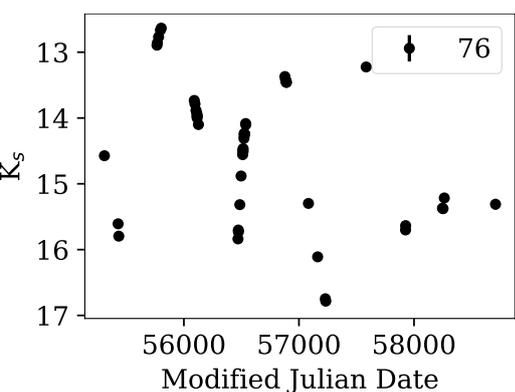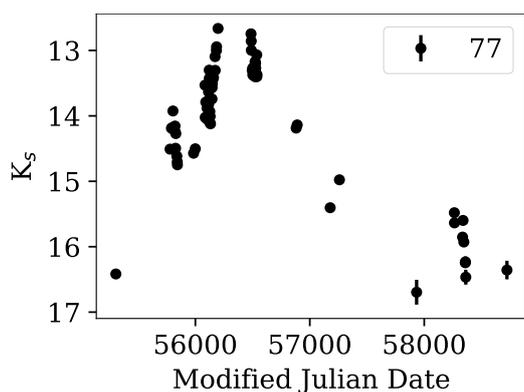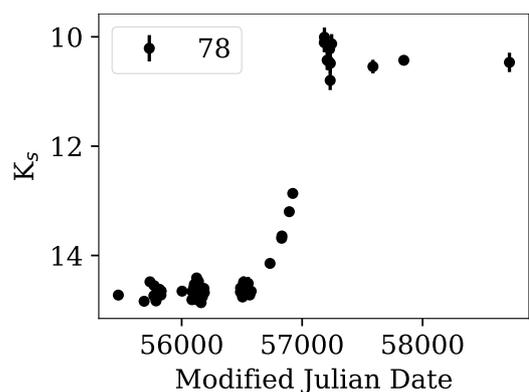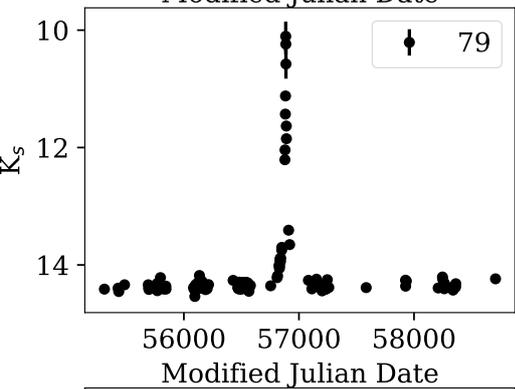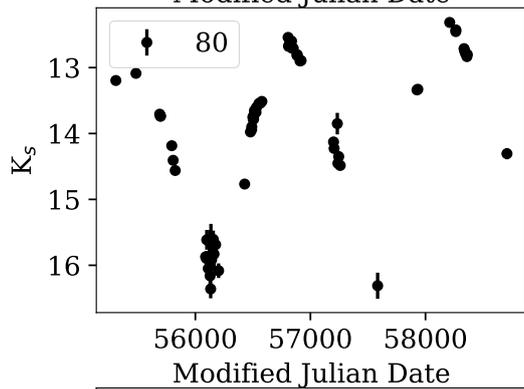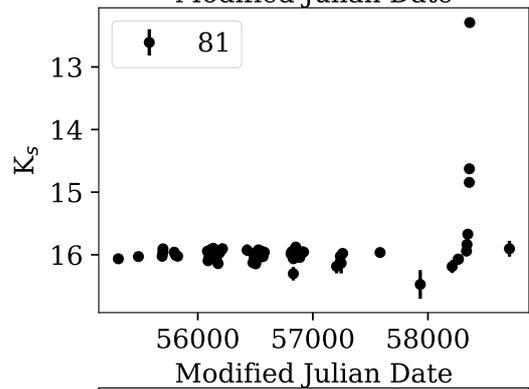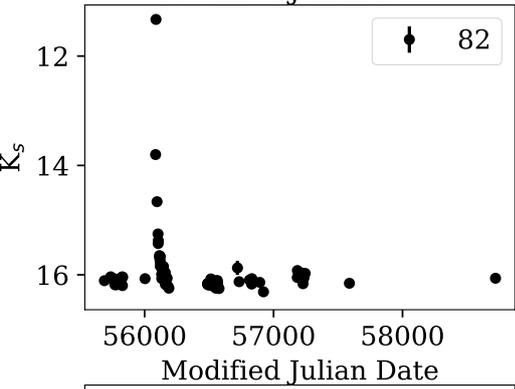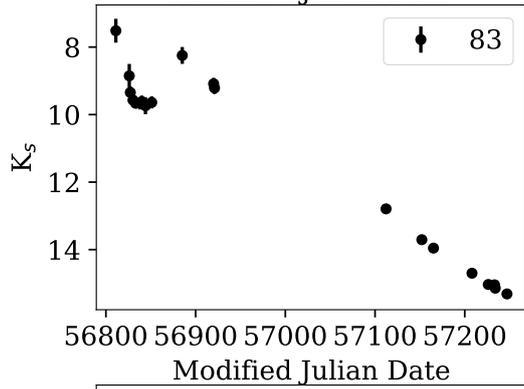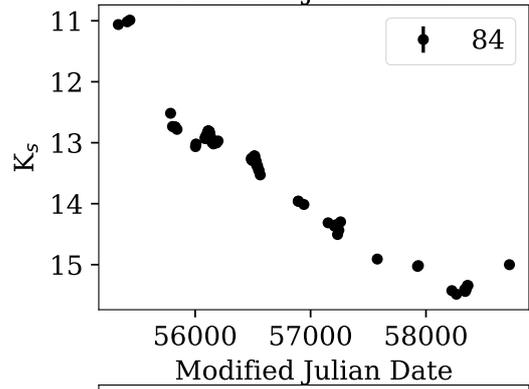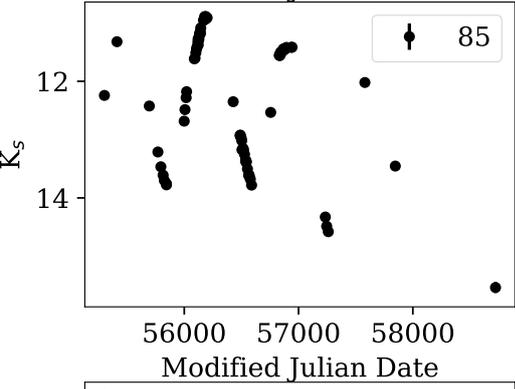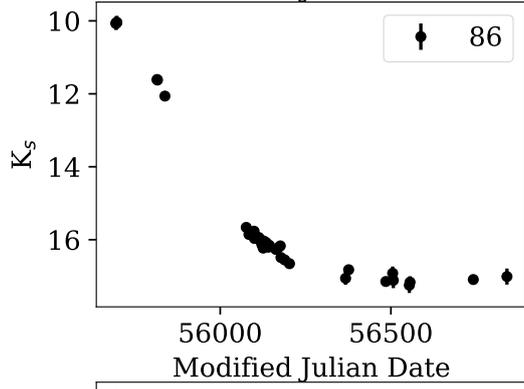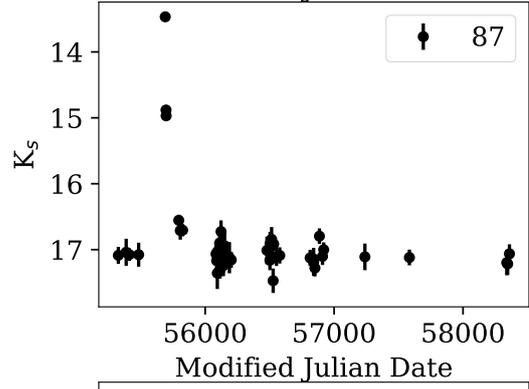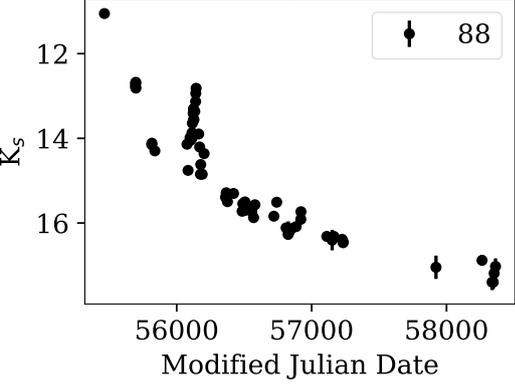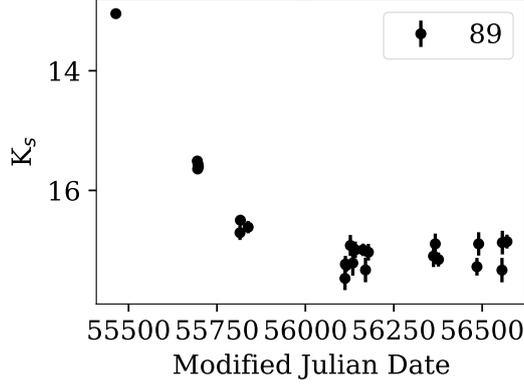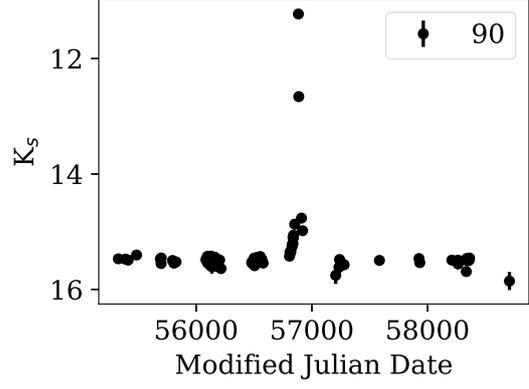

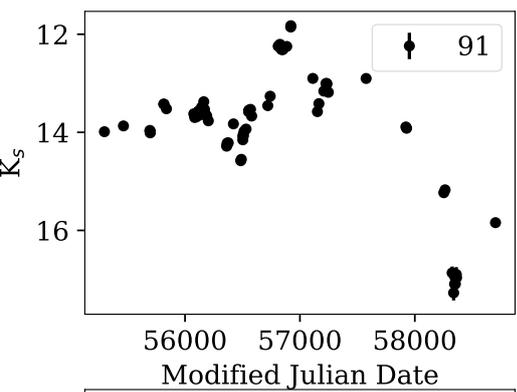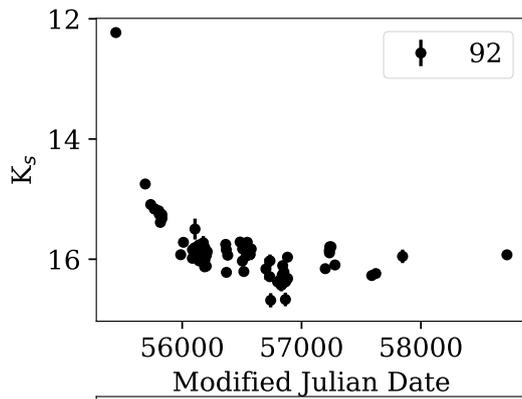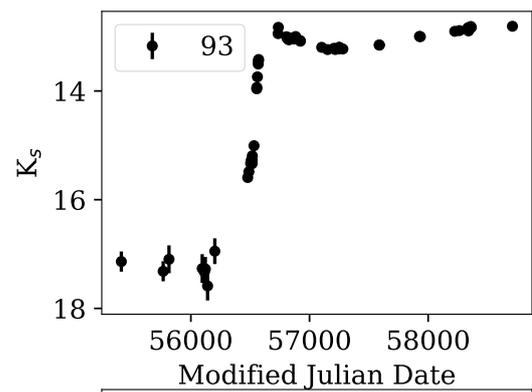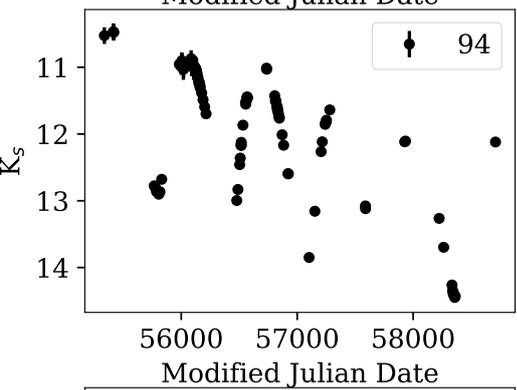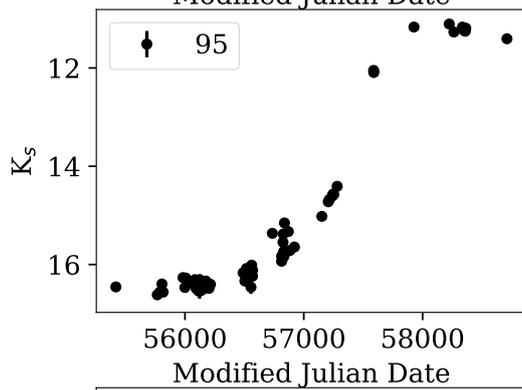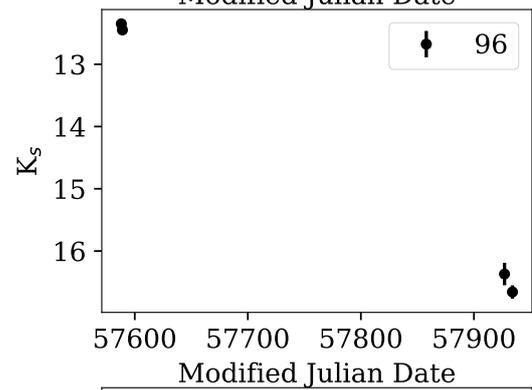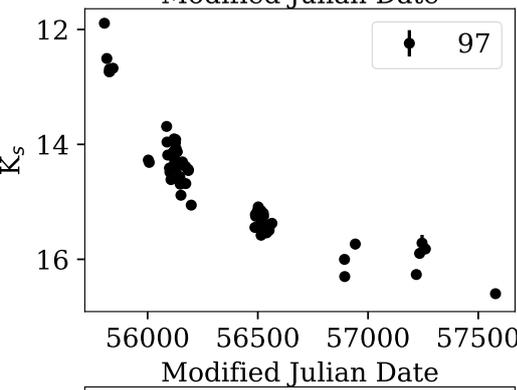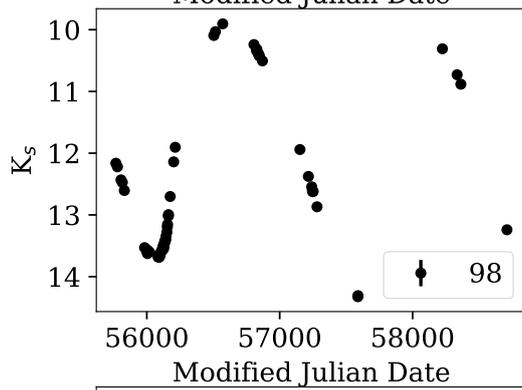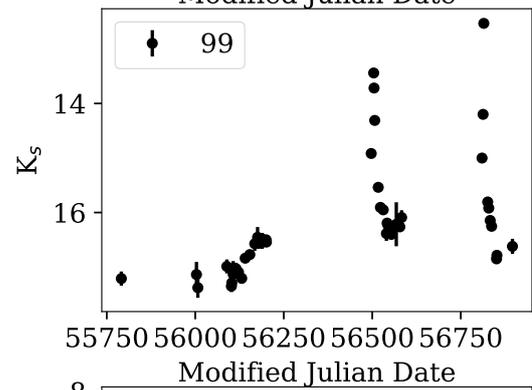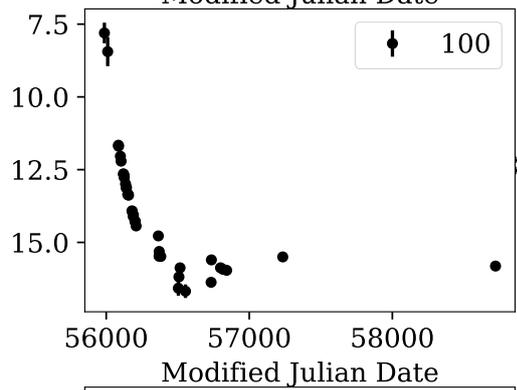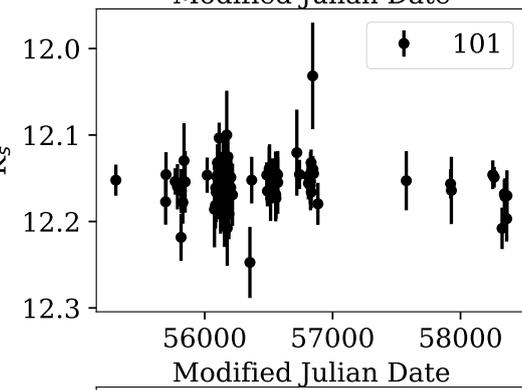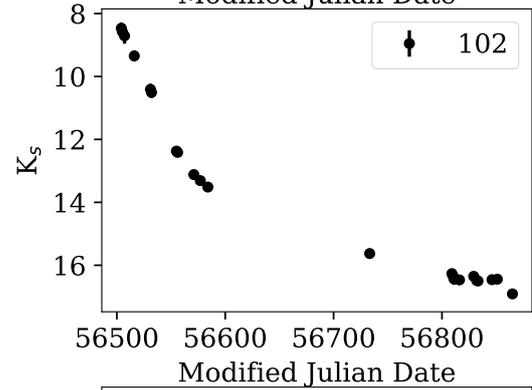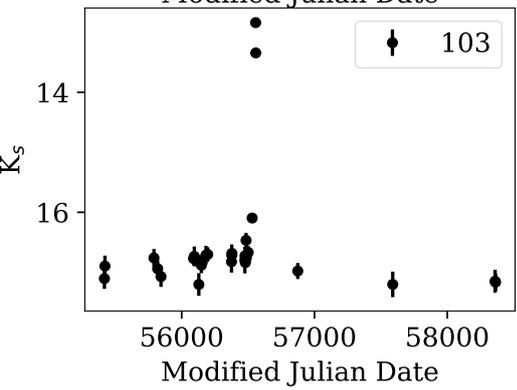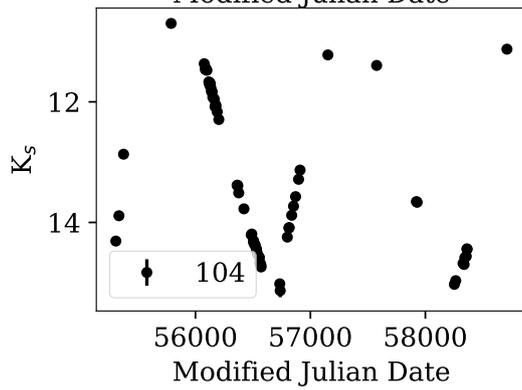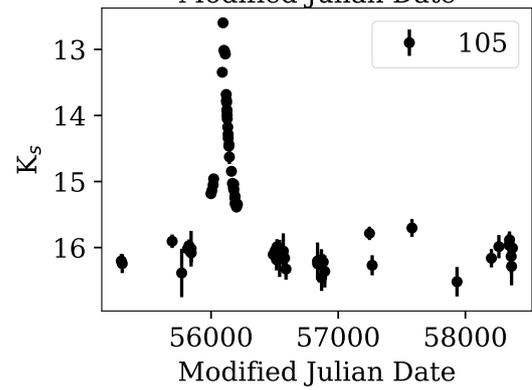

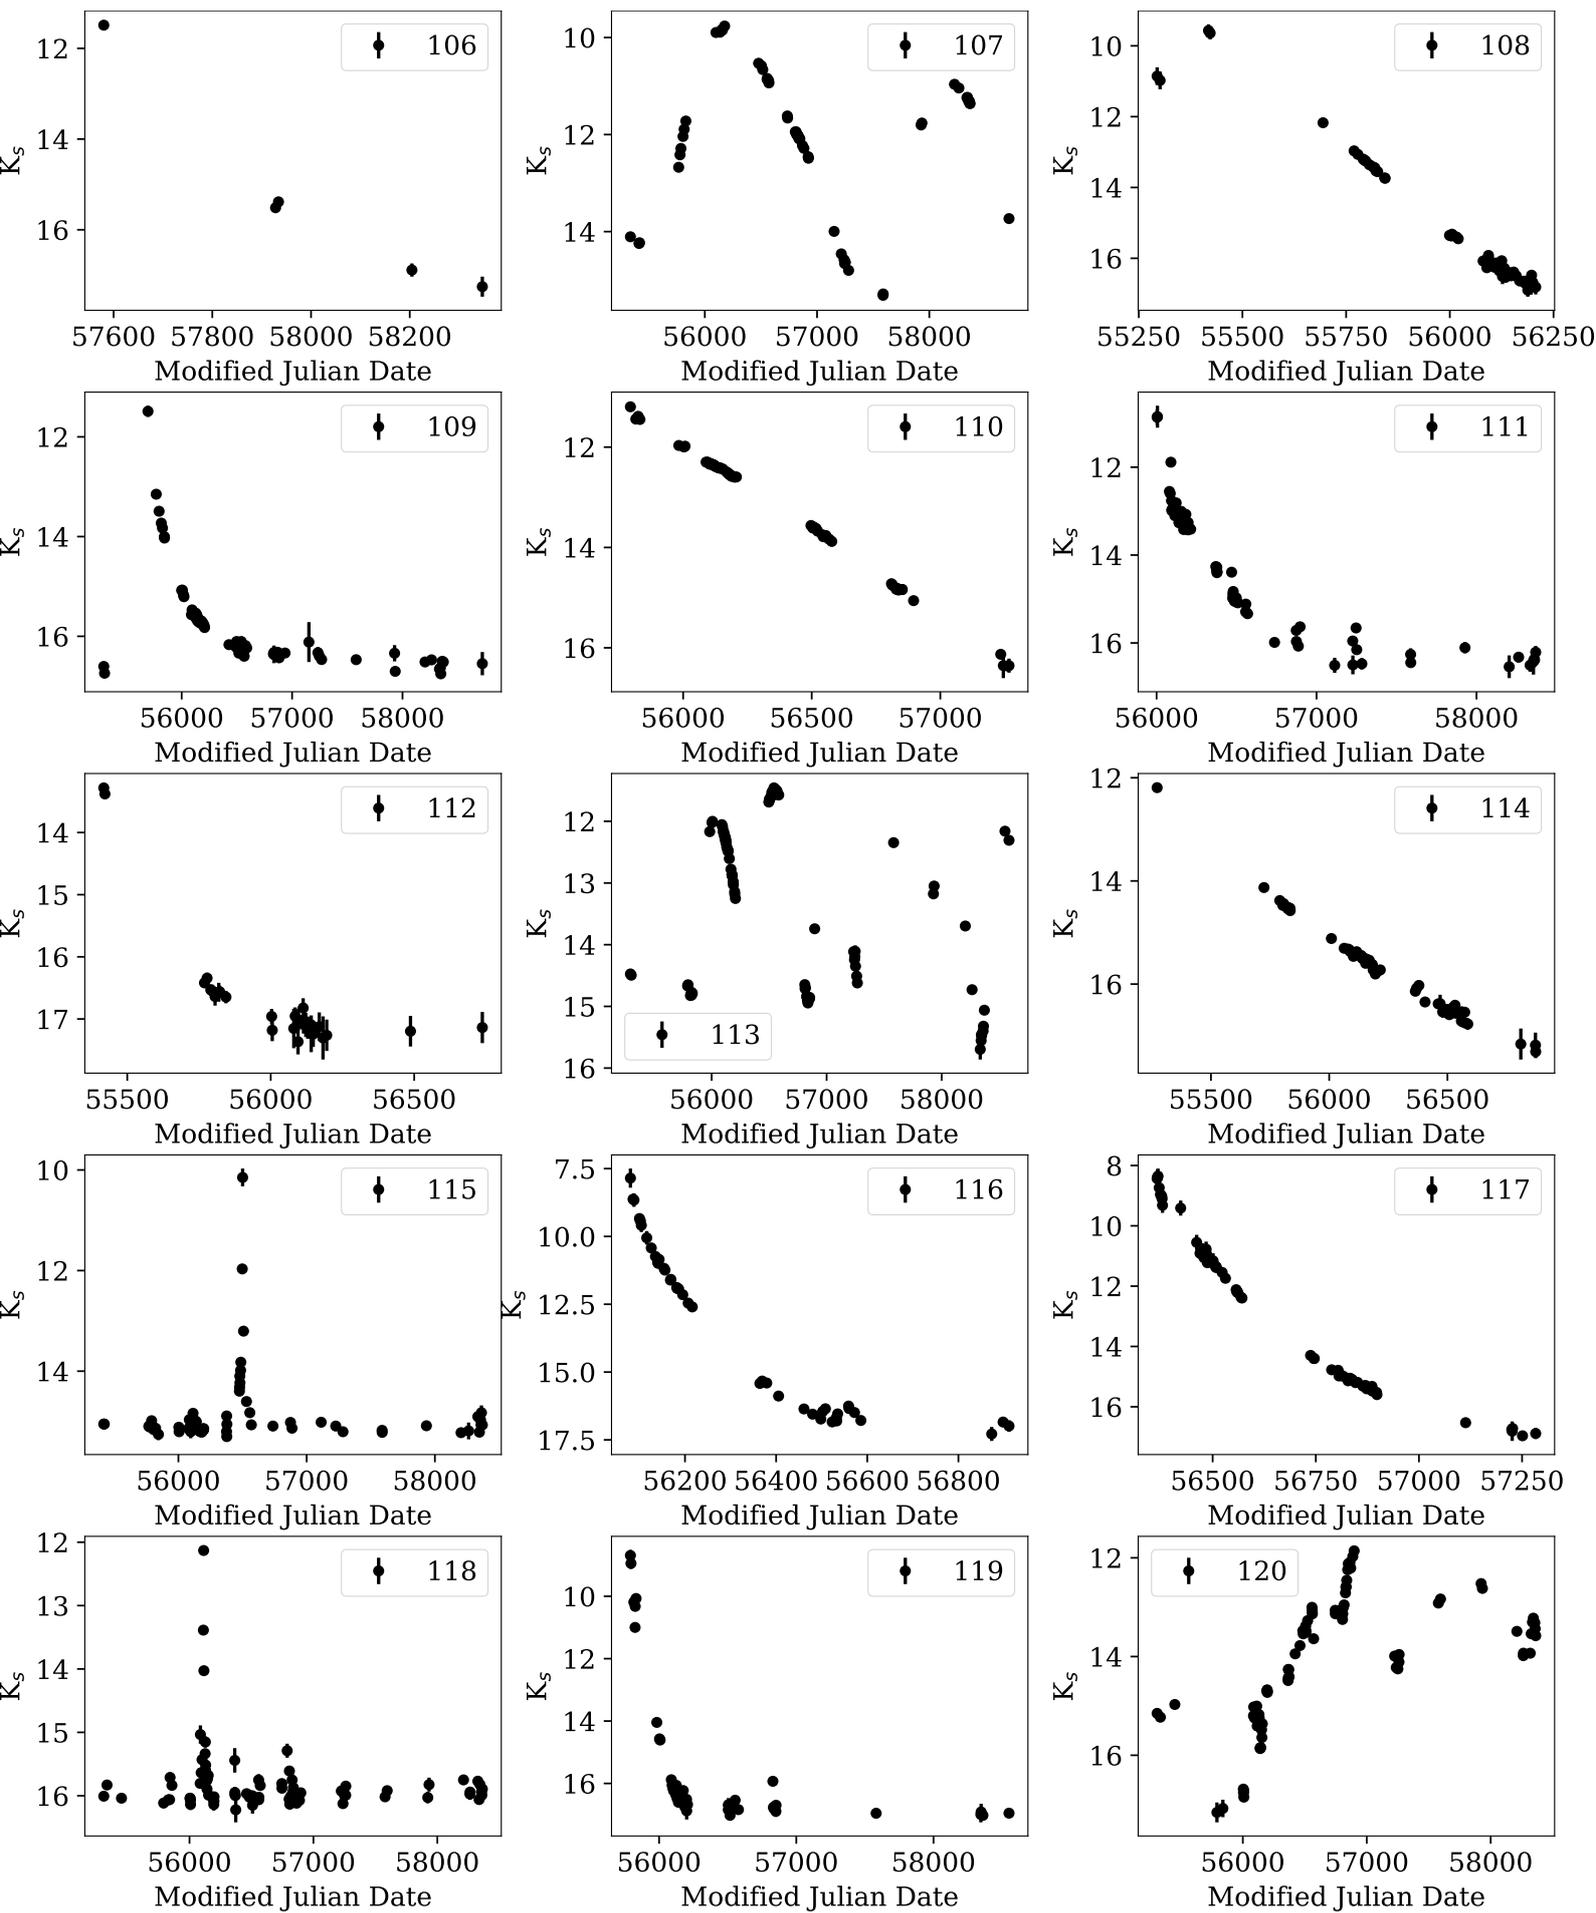

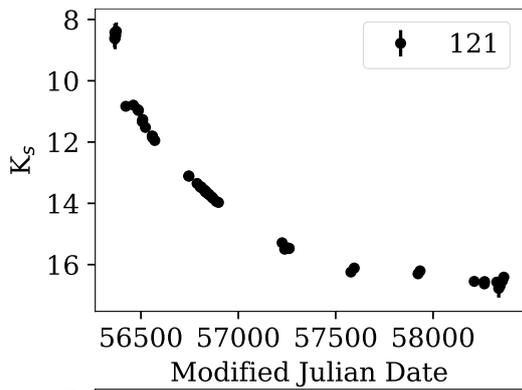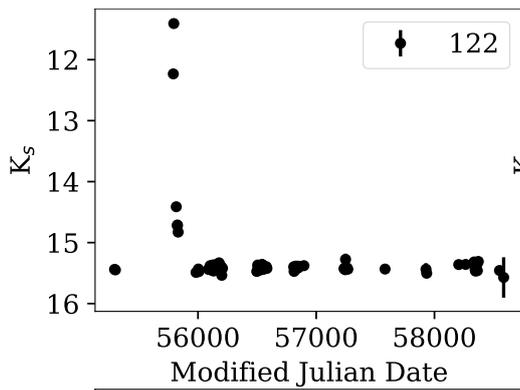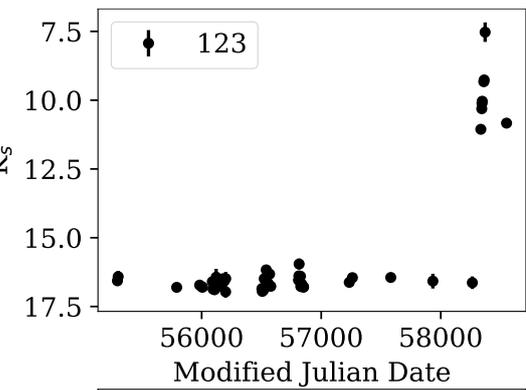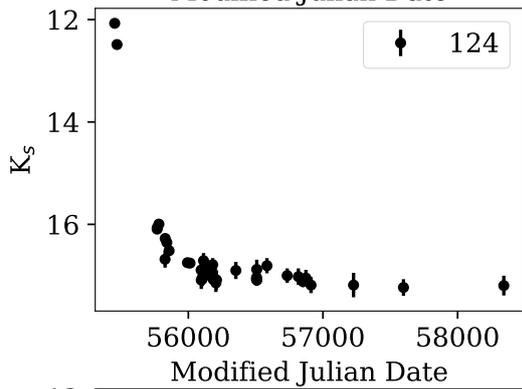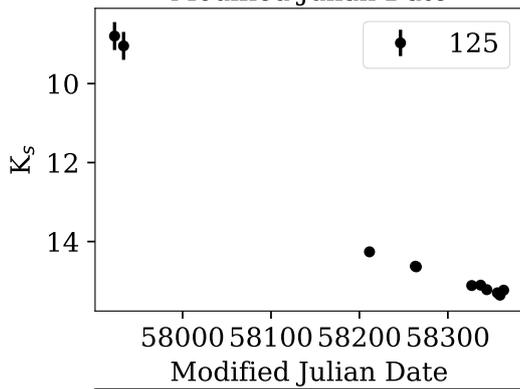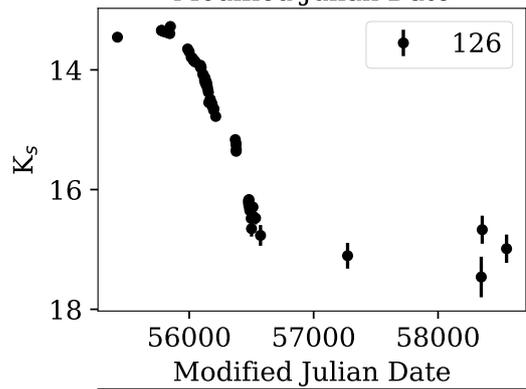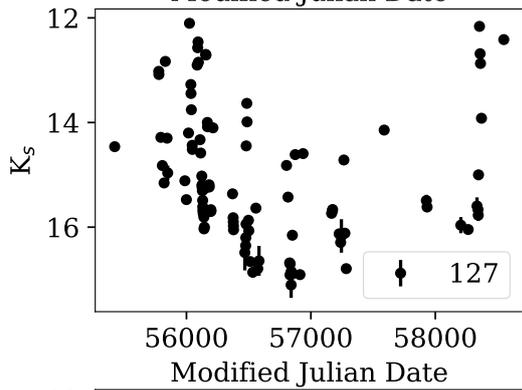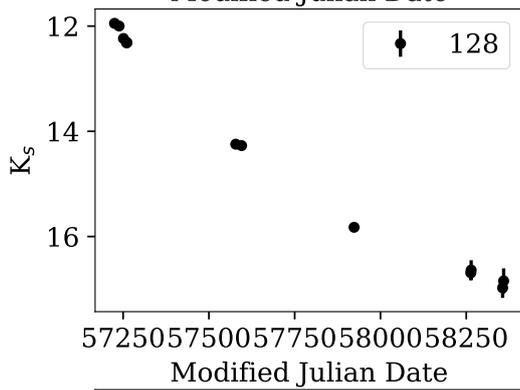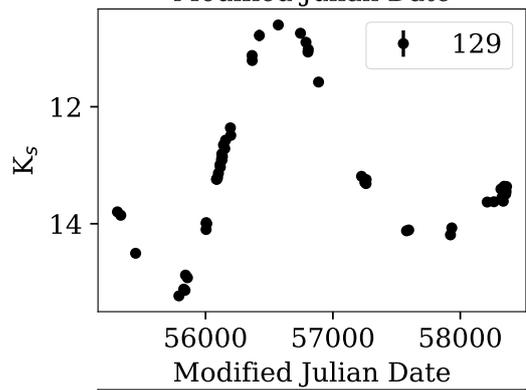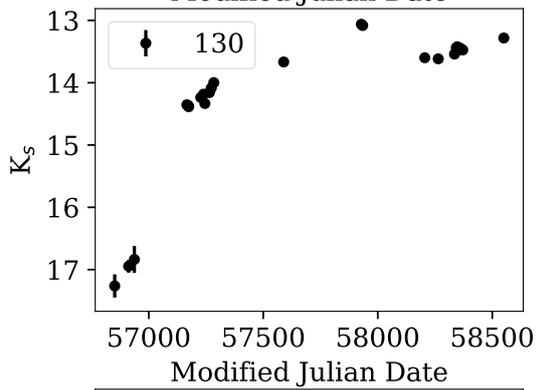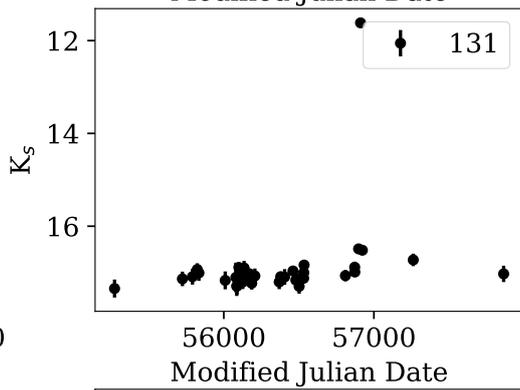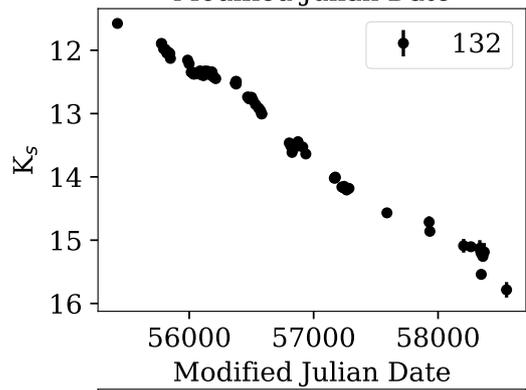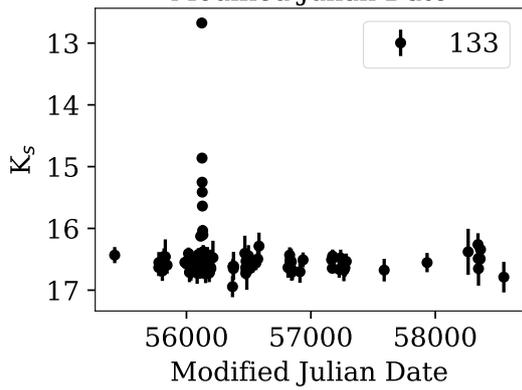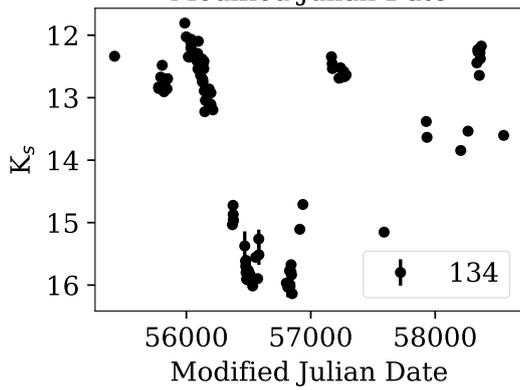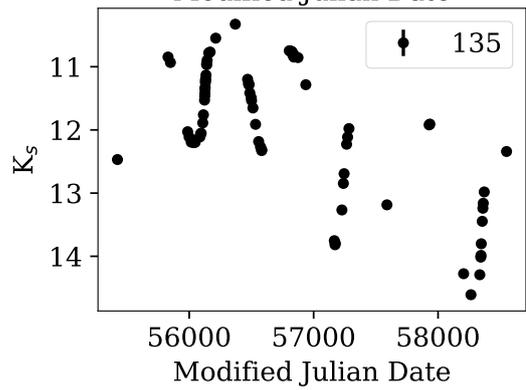

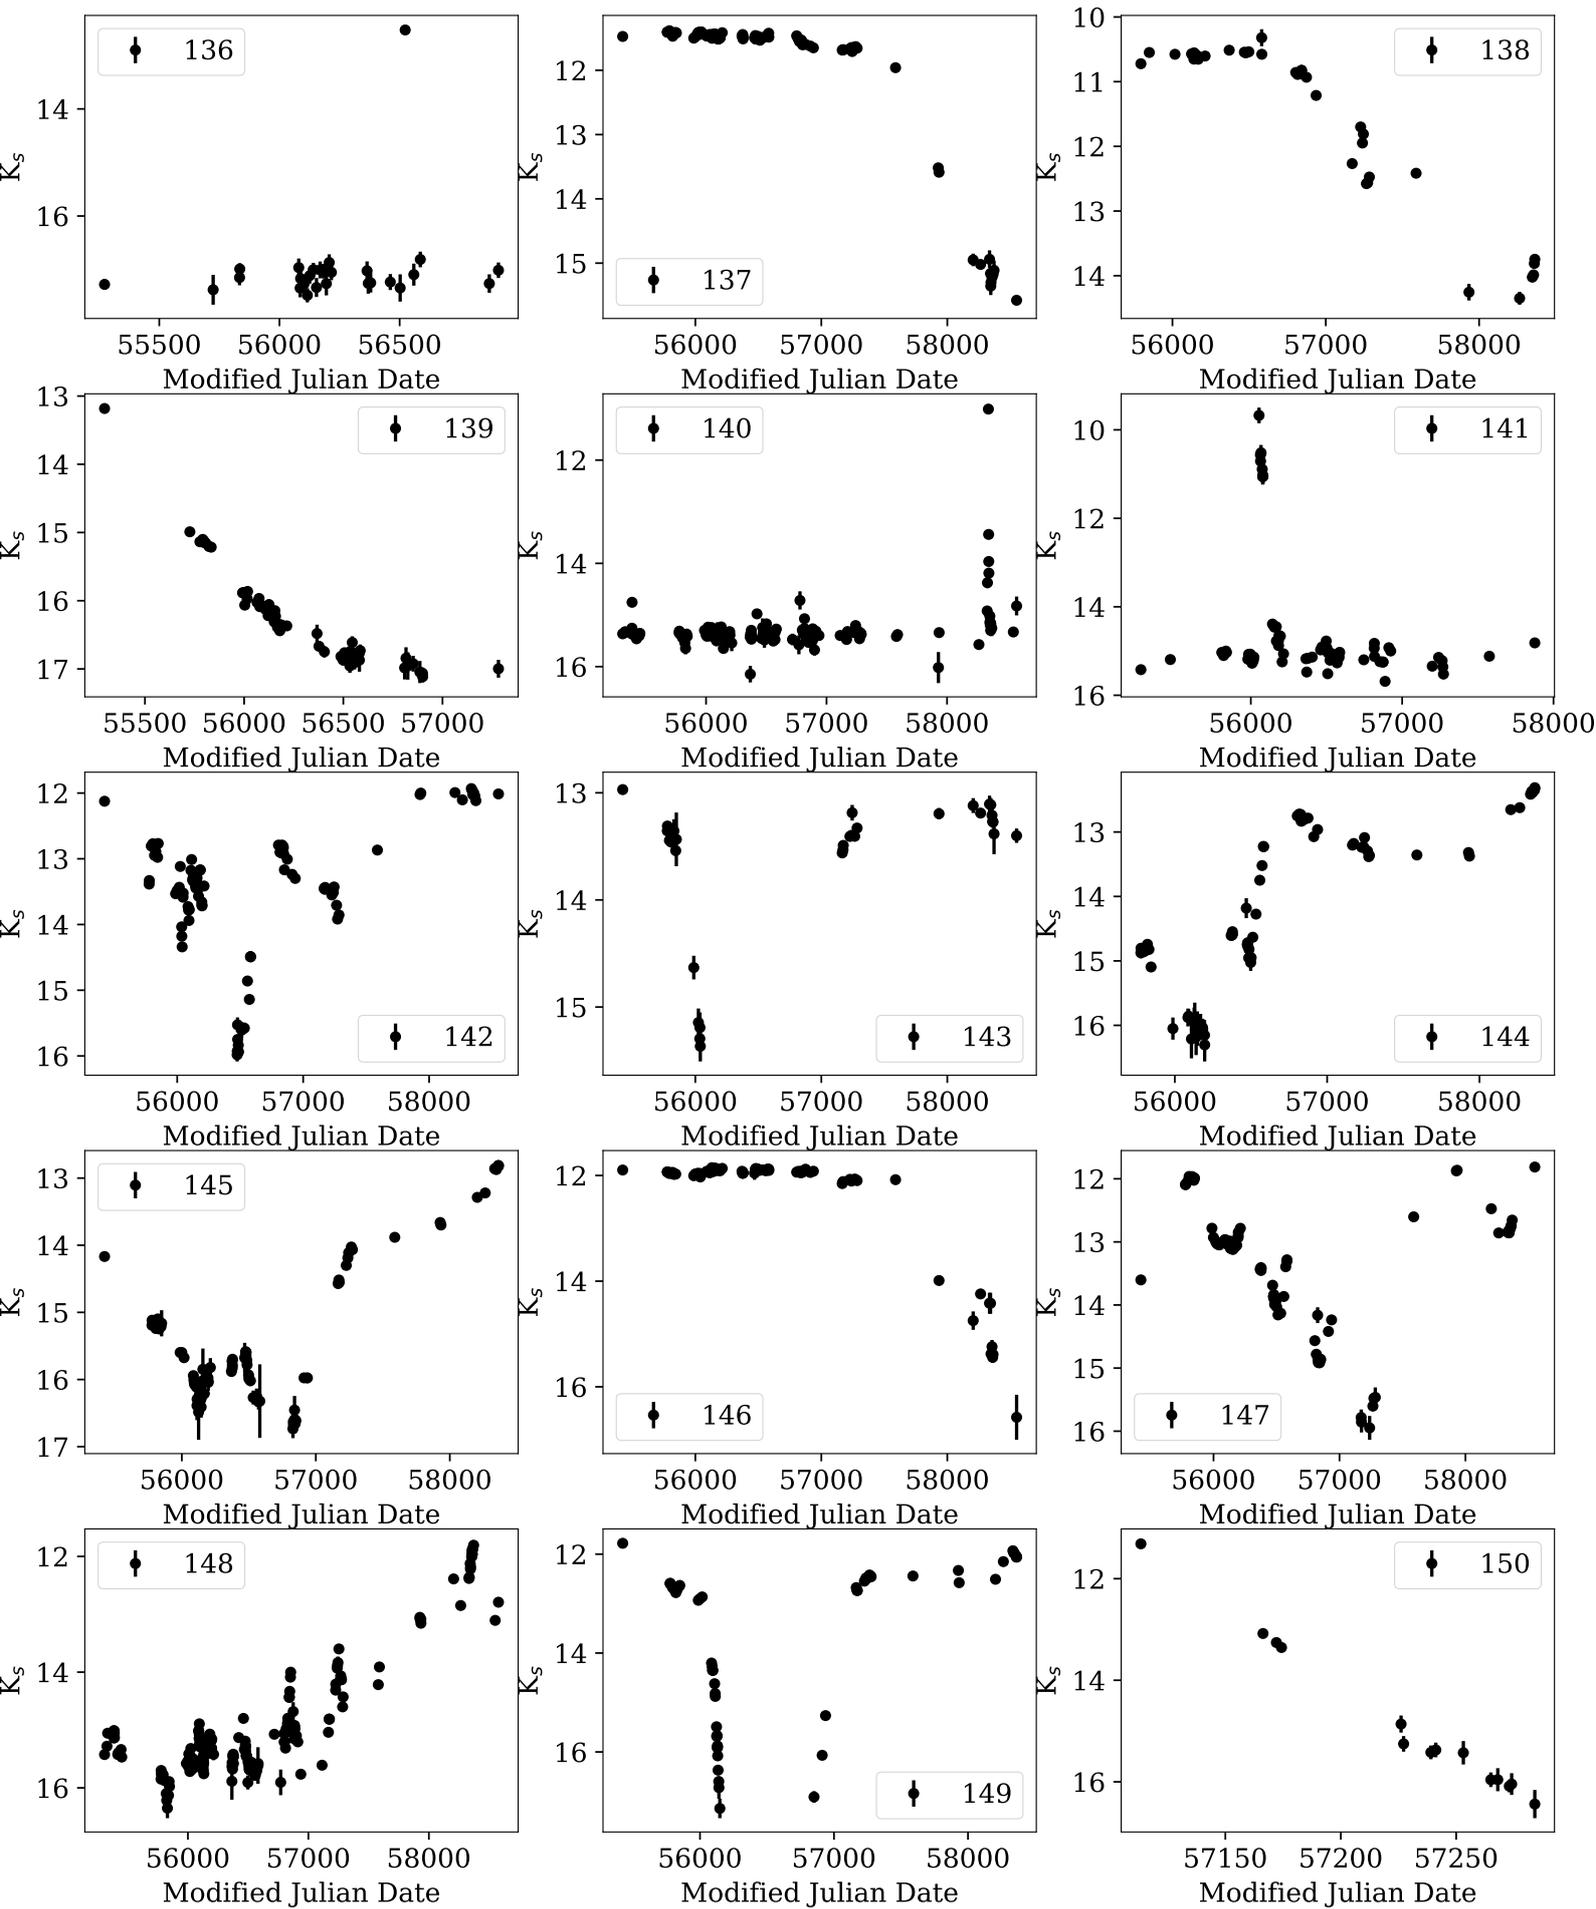

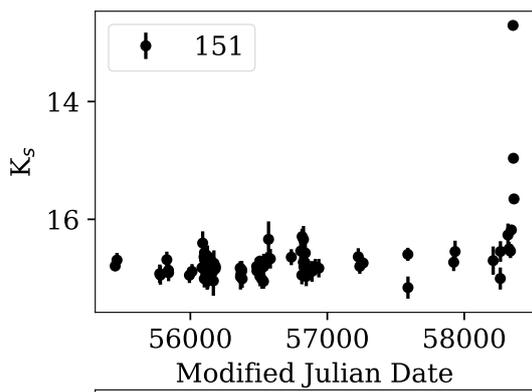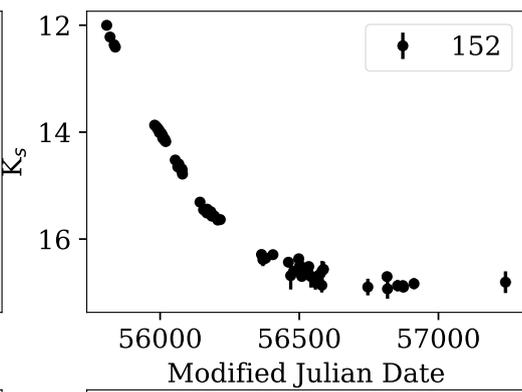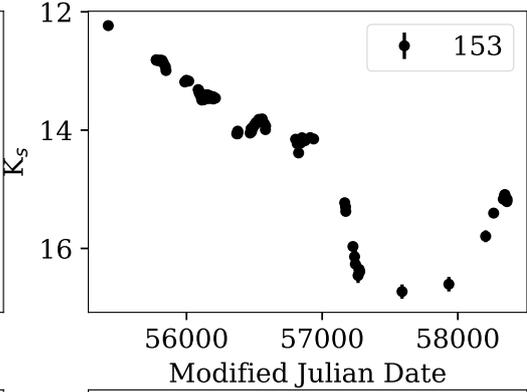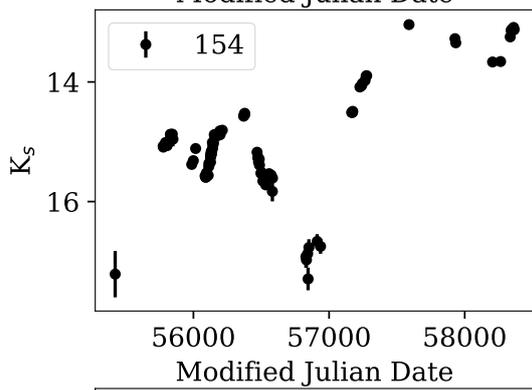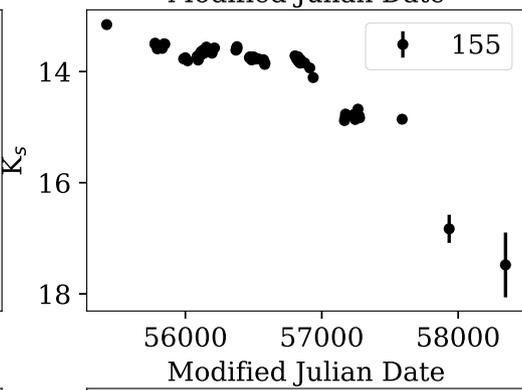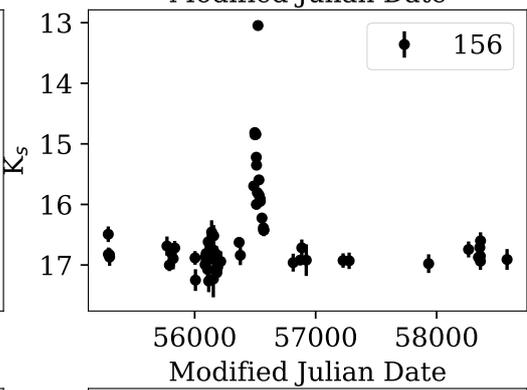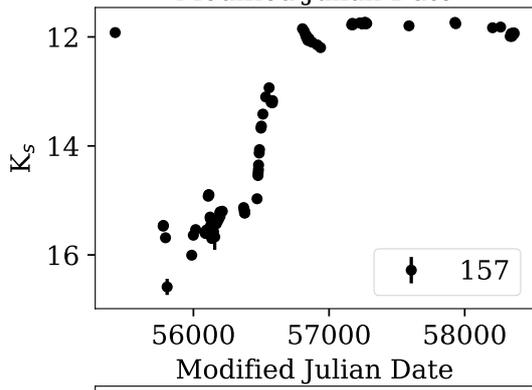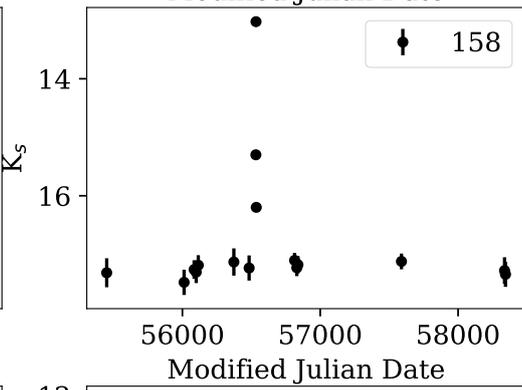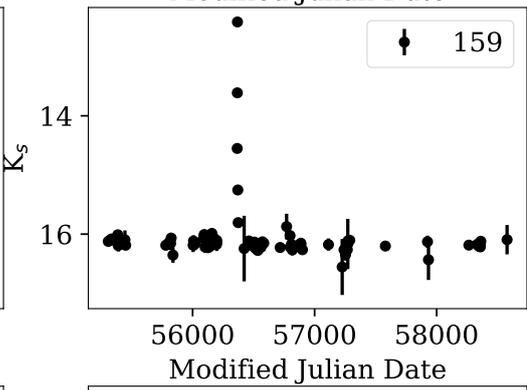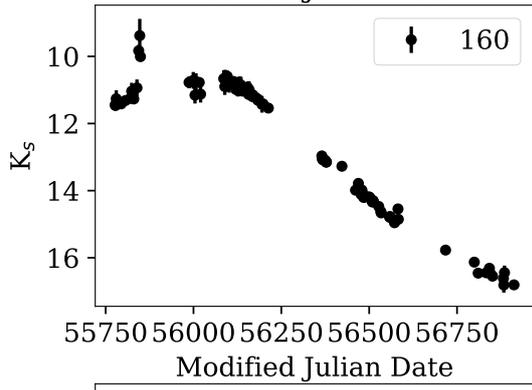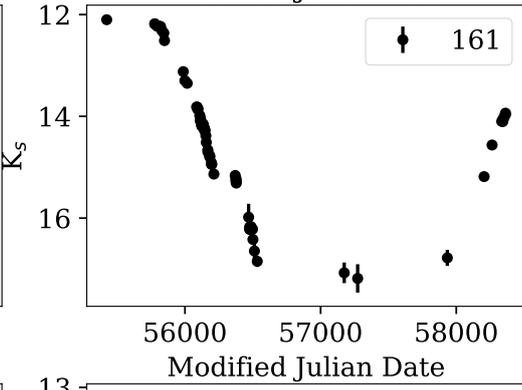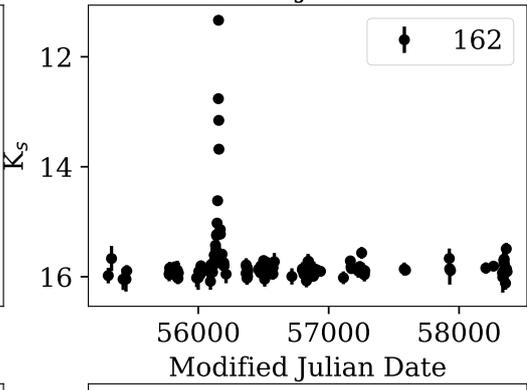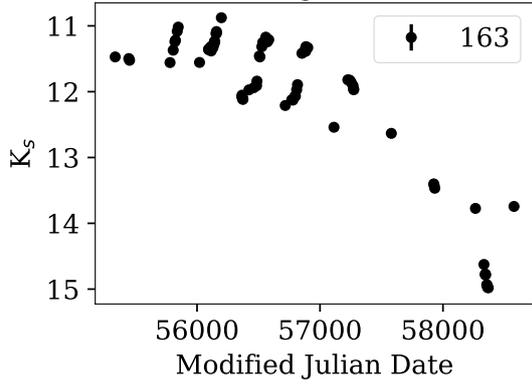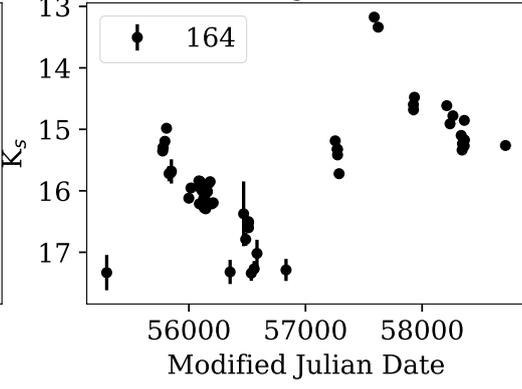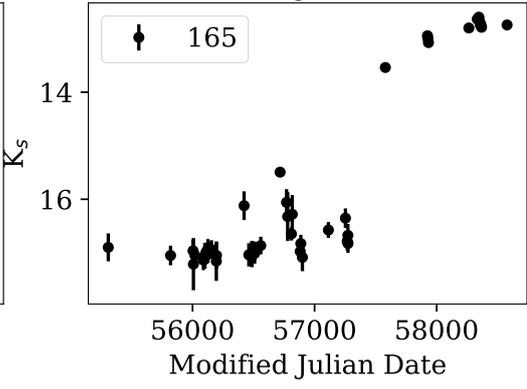

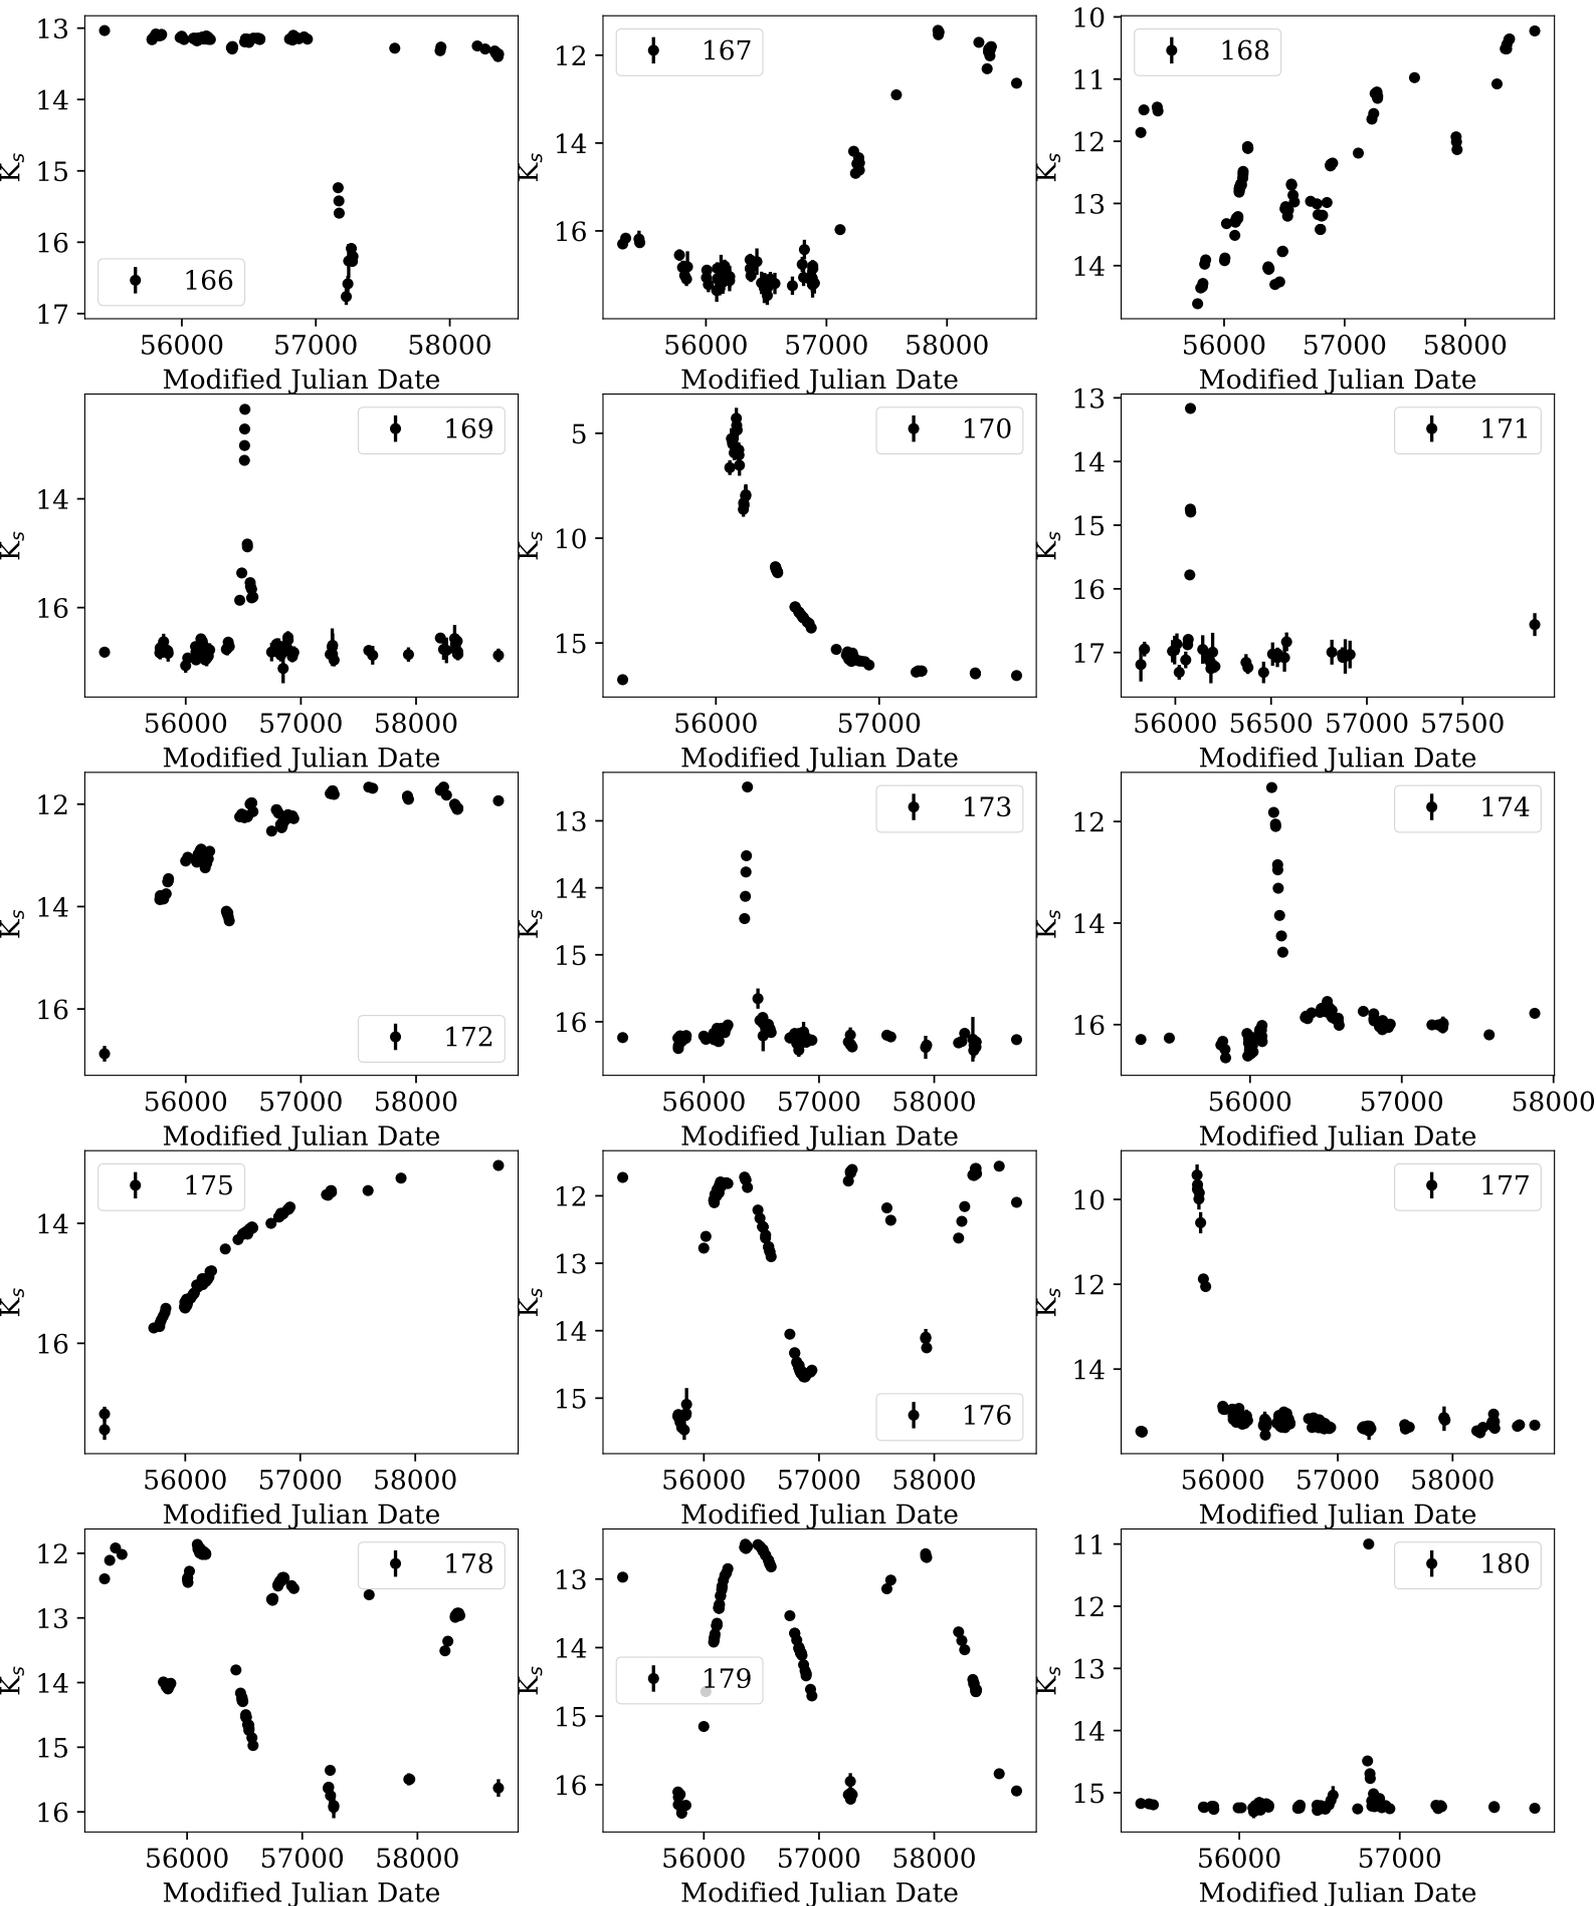

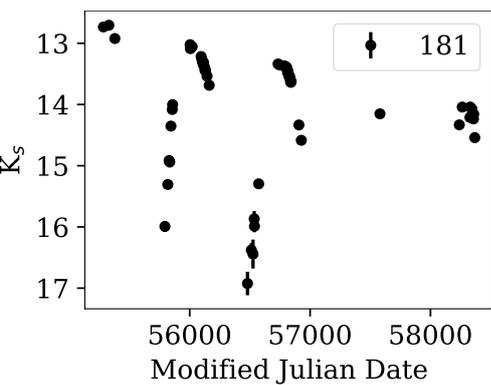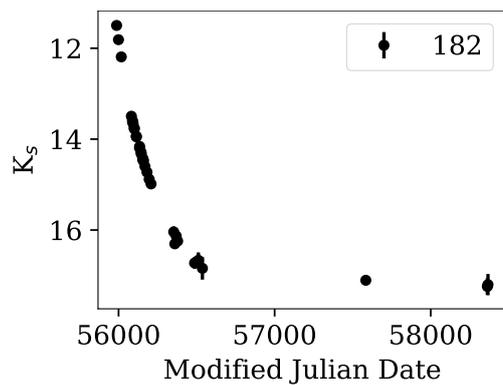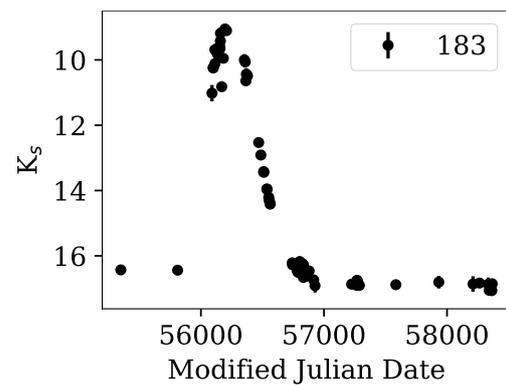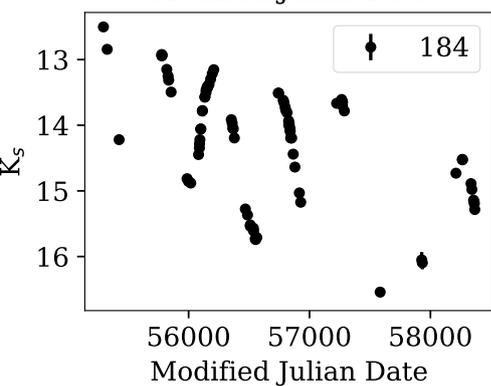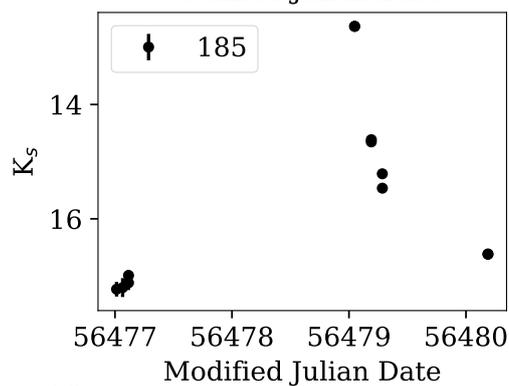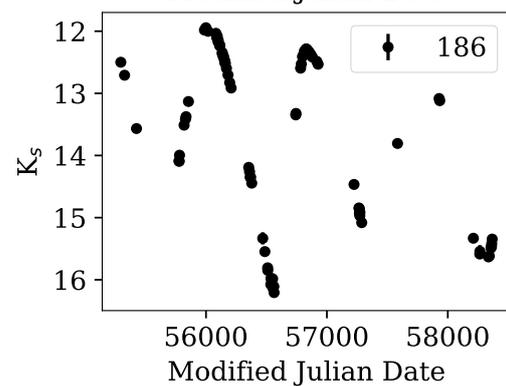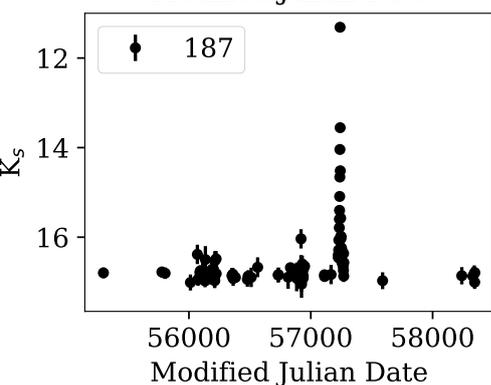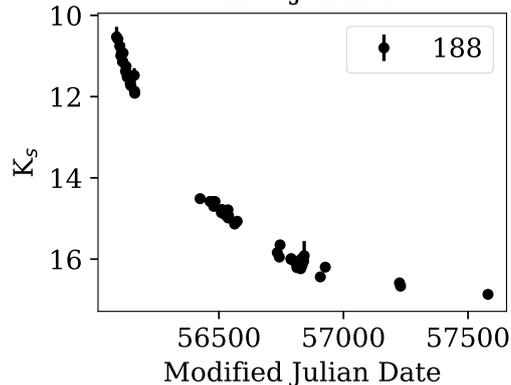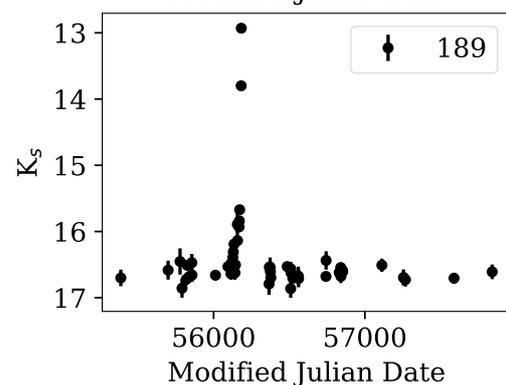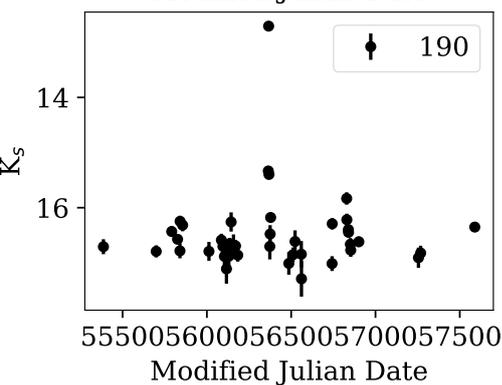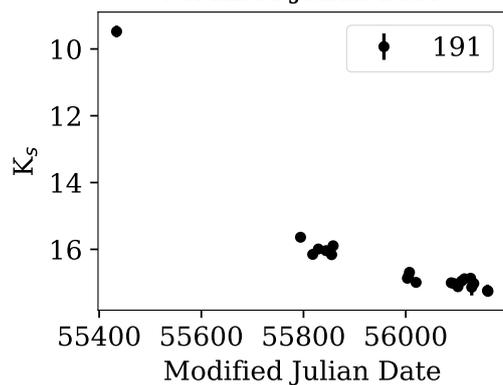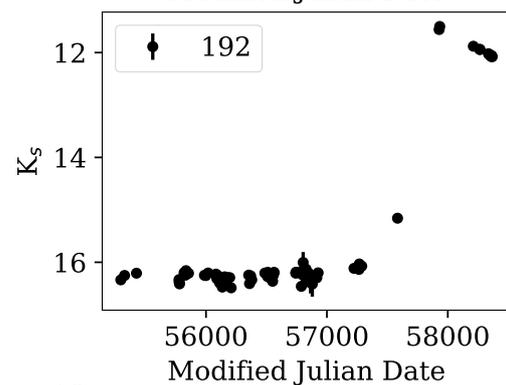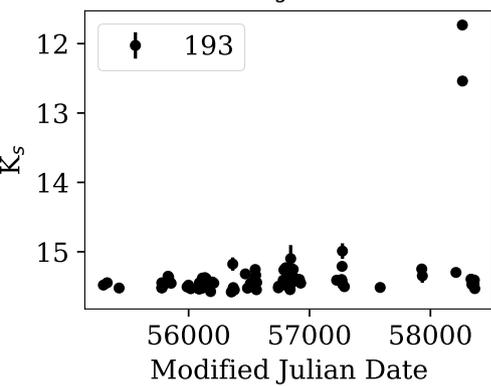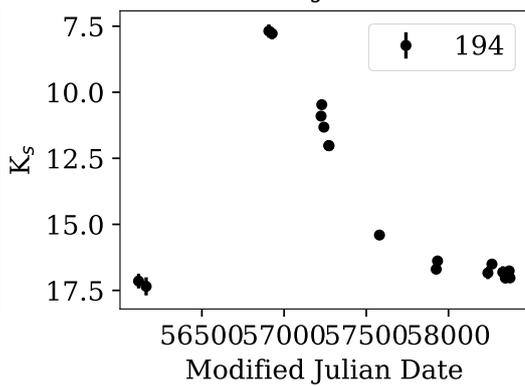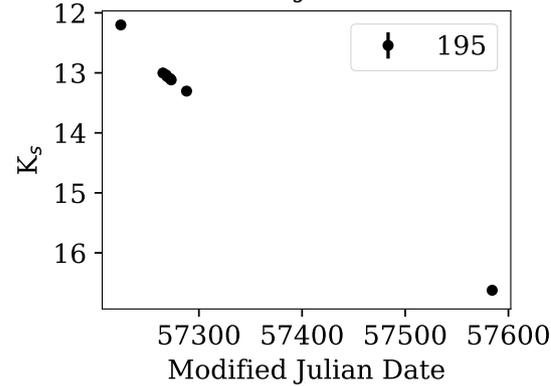

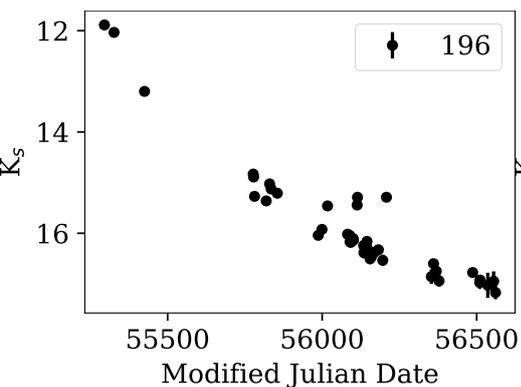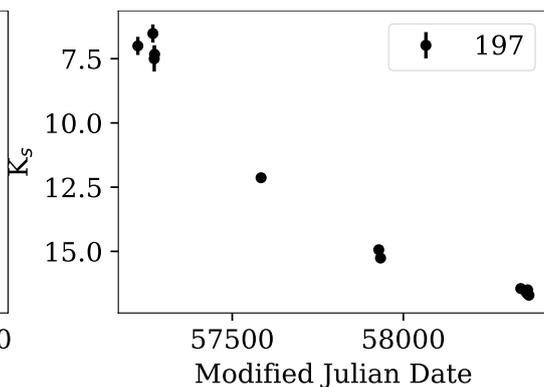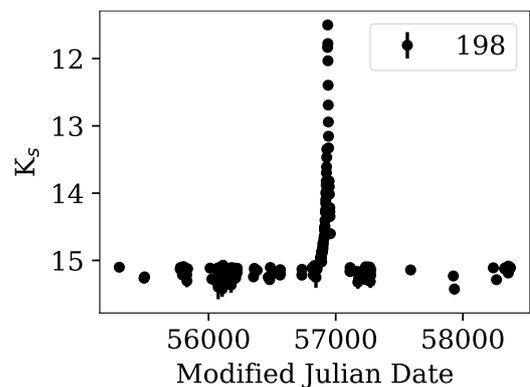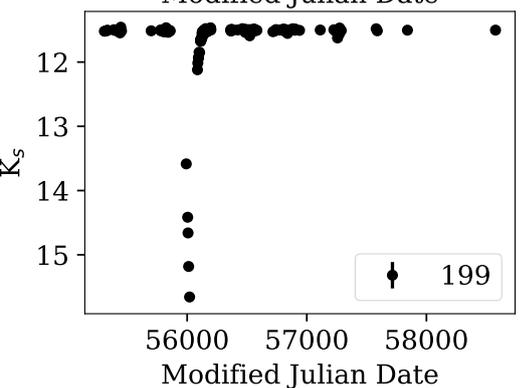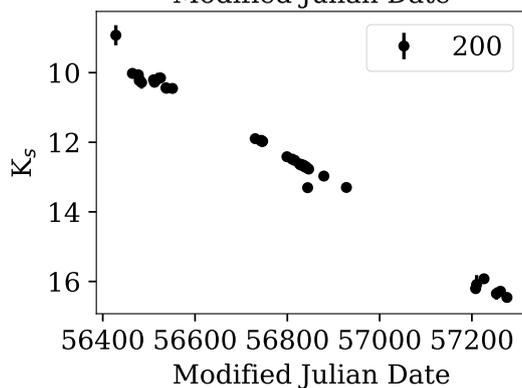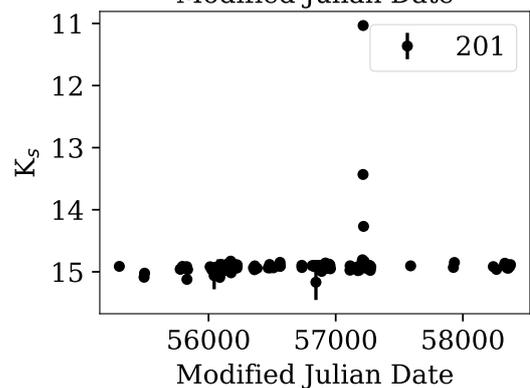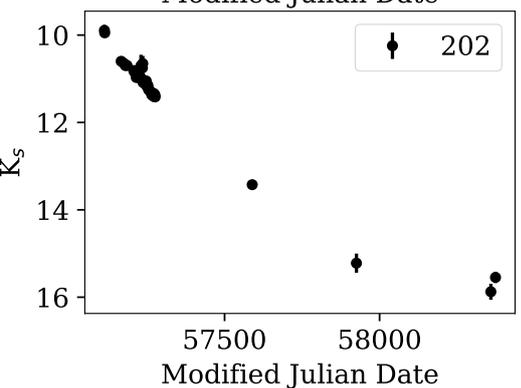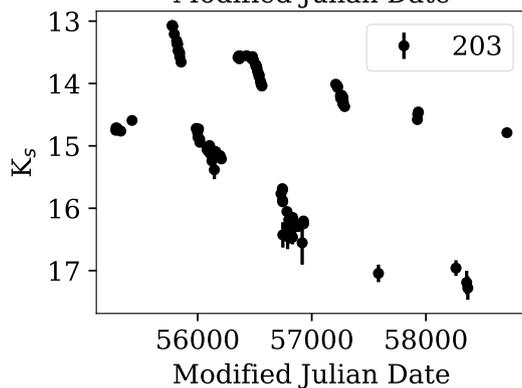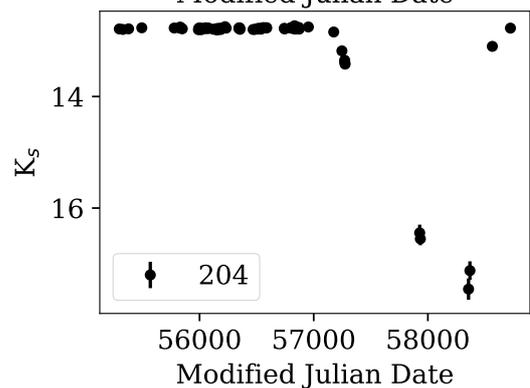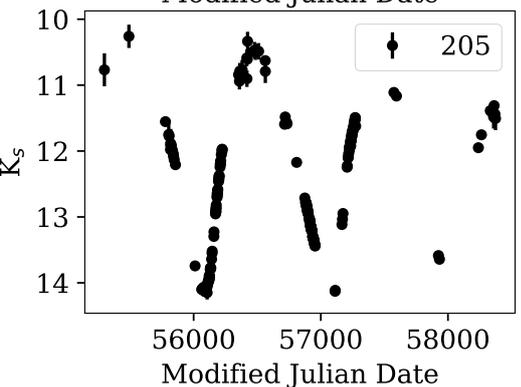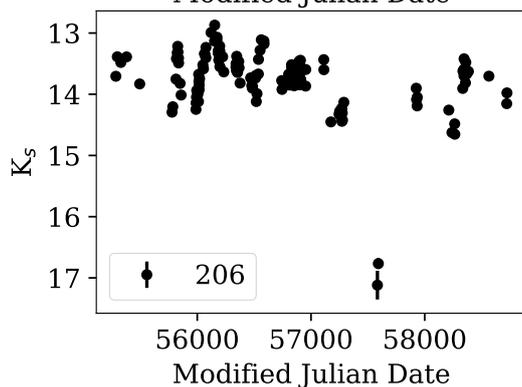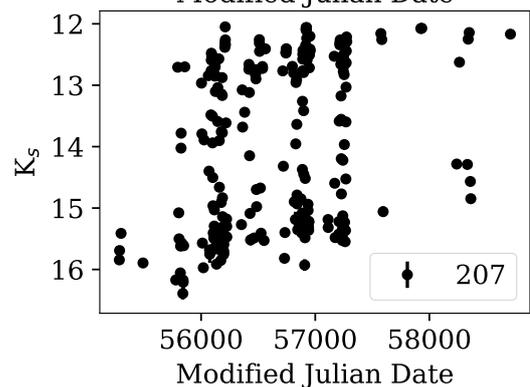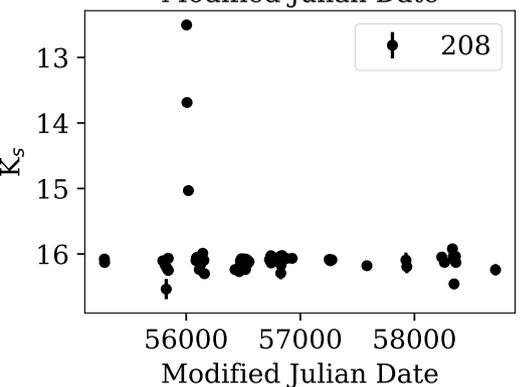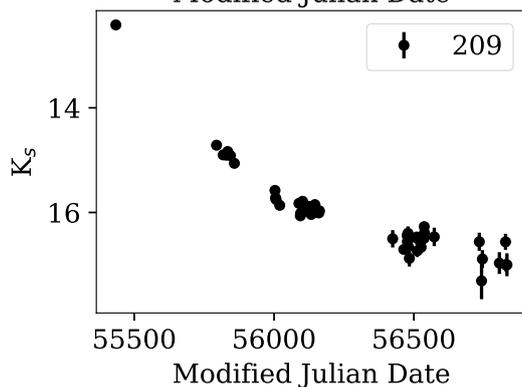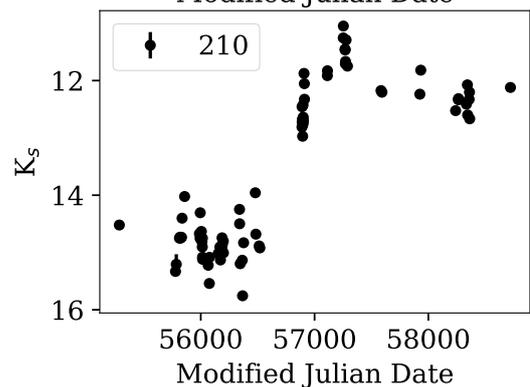

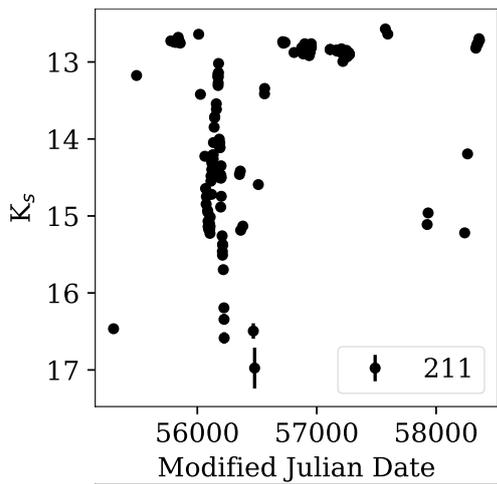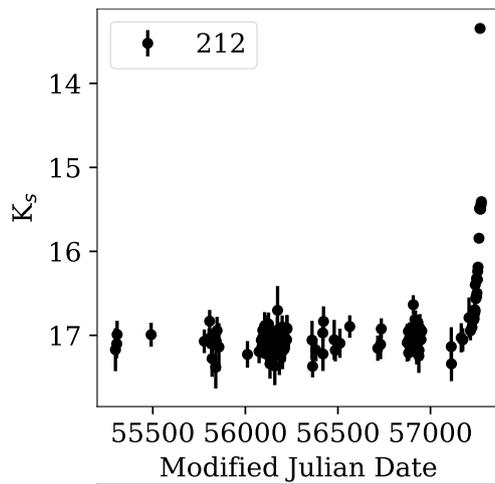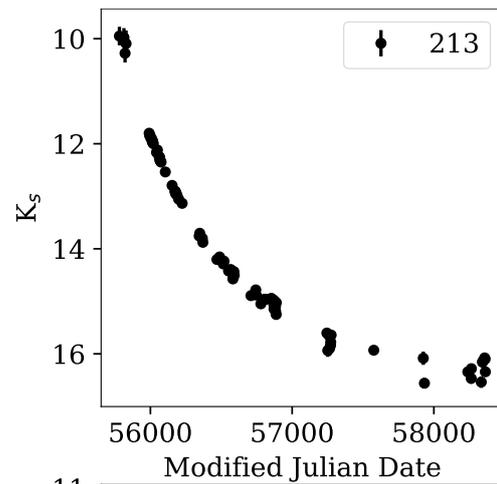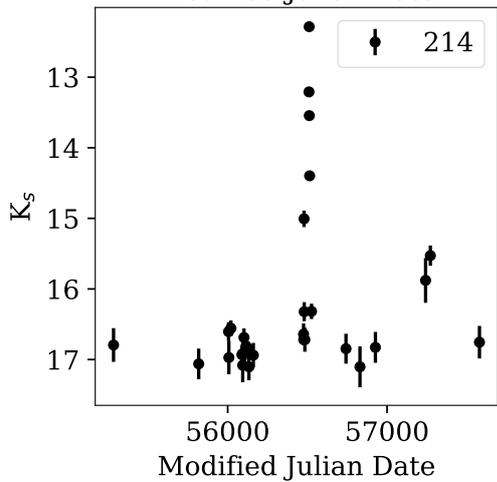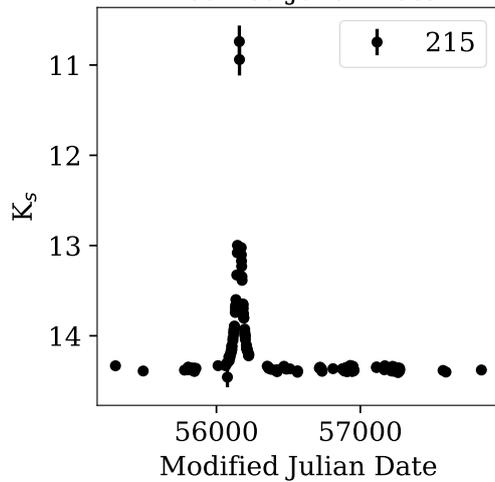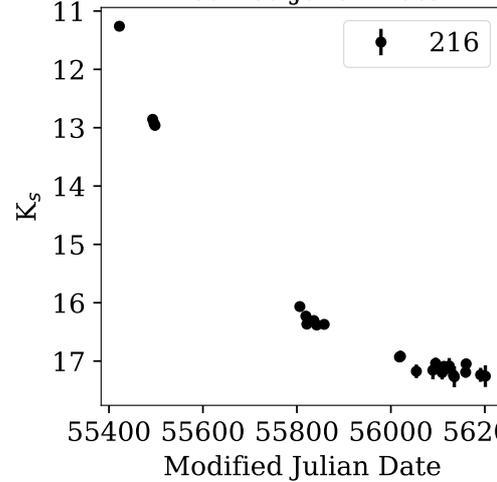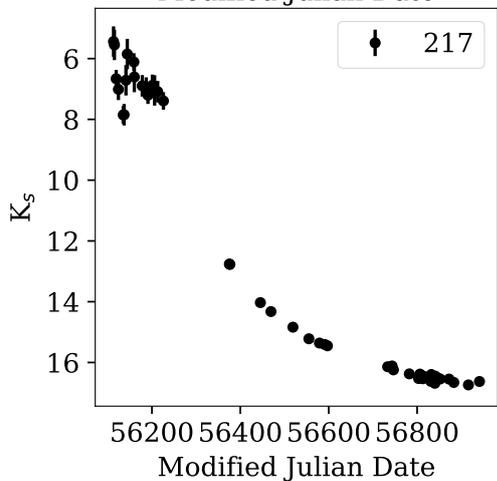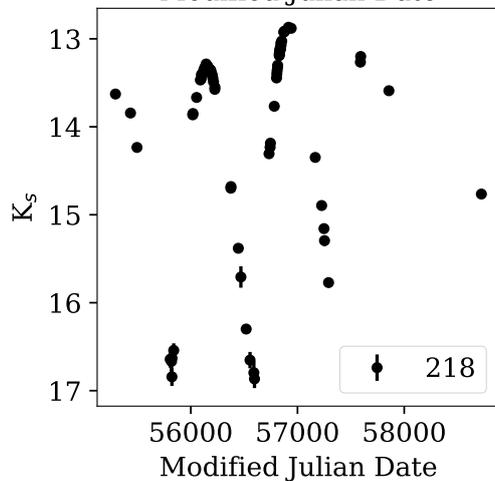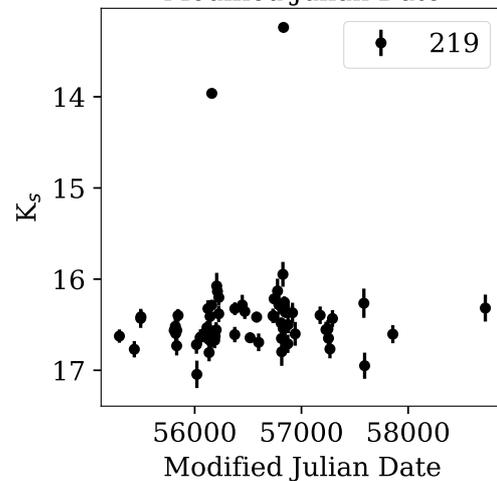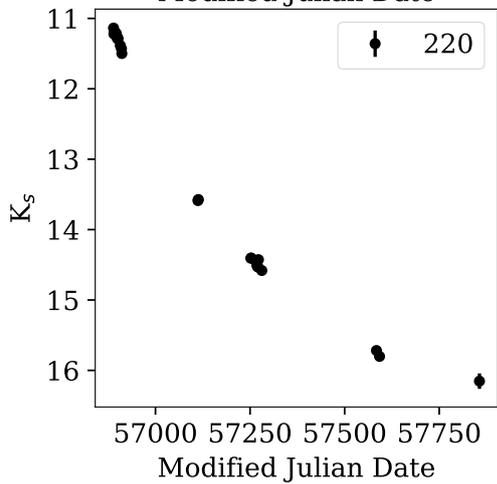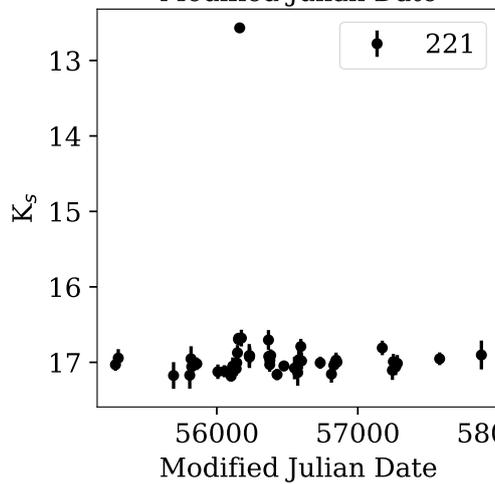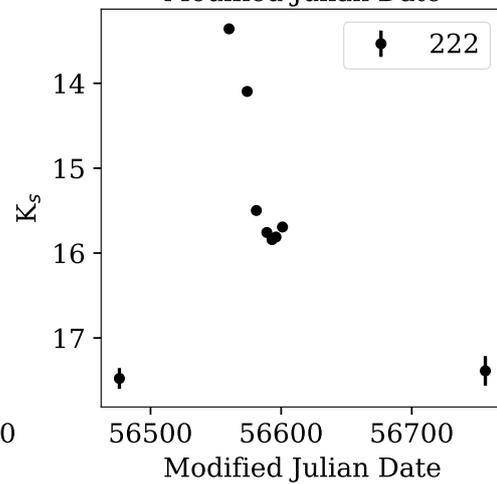

Supplement: Supplementary file 2 [file LCs_all.pdf]
